# Supplementary material for: arrayMap: A Reference Resource for Genomic Copy Number Imbalances in Human Malignancies
Source: arXiv:1201.2677 ancillary file (2012-01-11)
Supplement: Supplementary file 1 [file 20120111_Cai_Kumar_Baudis_arrayMap_supplement1.pdf]

[Search Public Series](#)[Search Public Arrays](#)[Plot Array Data](#)[Progenetix](#)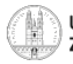**University of  
Zurich**[News](#)[Citation](#)[FAQ & Guide](#)[Contributing Authors](#)[CompBio Zurich](#)[Atlas of Cytogenetics in  
Hematology/Oncology](#)[NCI SKY/M-FISH and  
CGH Database](#)[NCI Cancer Chromosomes](#)[FOLLOW US ON !\[\]\(4f6bf54ae7e4144a72d78316053e412d\_img.jpg\)](#)[Share !\[\]\(3342c215b2a8b663596a81468d5dc314\_img.jpg\) !\[\]\(5e22d44aef1f9548ca8274cbfb388e9d\_img.jpg\) !\[\]\(b011182daf5a0527ed818f91dc4cf8f7\_img.jpg\) !\[\]\(e021942709a217cfed2f781c62feb09c\_img.jpg\) !\[\]\(189fbc627457efb1015bb006253636f9\_img.jpg\)](#)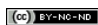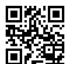

130.60.44.246

130.60.93.222

Visualization of genomic array data sets 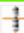 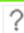

|                                                                                      |                                                                                    |                                     |                                                     |     |
|--------------------------------------------------------------------------------------|------------------------------------------------------------------------------------|-------------------------------------|-----------------------------------------------------|-----|
| SERIES                                                                               | <input type="text" value="GSE21530"/>                                              |                                     |                                                     | [?] |
| ARRAY ID                                                                             | <input type="text"/>                                                               |                                     |                                                     | [?] |
| <input type="button" value="Show original plots &amp; Load defaults (if existing)"/> |                                                                                    |                                     |                                                     |     |
| CASE DATA PLOTTING                                                                   | <input type="text" value="no plot refresh"/>                                       |                                     |                                                     | [?] |
| GOLDEN PATH EDITION                                                                  | <input type="text" value="HG18 / 36"/>                                             |                                     |                                                     | [?] |
| PLOT REGION                                                                          | <input type="text"/>                                                               |                                     |                                                     | [?] |
| CHROMOSOMES TO PLOT                                                                  | <input type="text" value="1:22"/>                                                  |                                     |                                                     | [?] |
| LOSS/GAIN THRESHOLDS                                                                 | <input type="text" value="-0.15"/>                                                 | <input type="text" value="0.15"/>   | Y AXIS FACTOR <input type="text" value="1.2"/>      | [?] |
| REGION SIZE                                                                          | <input type="text" value="0"/>                                                     | <input type="text" value="250000"/> | MIN. PROBES <input type="text" value="2"/>          | [?] |
| EMAIL / PASSWORD                                                                     | <input type="text" value="your registered email"/>                                 |                                     | <input type="text" value="your received password"/> | [?] |
| LICENSE AGREEMENT                                                                    | <input checked="" type="checkbox"/> I agree to license, disclaimer & citation note |                                     |                                                     |     |
| <input type="button" value="Filter / replot array data"/>                            |                                                                                    |                                     |                                                     |     |

8 will be processed.

|           |               |
|-----------|---------------|
| GSM537760 | 360 segments  |
| GSM537761 | 219 segments  |
| GSM537762 | 177 segments  |
| GSM537763 | 93 segments   |
| GSM537764 | 1178 segments |
| GSM537765 | 392 segments  |
| GSM537766 | 69 segments   |
| GSM537767 | 341 segments  |

8 arrays were found.

parsing database ...

|                                    |                                                                                     |
|------------------------------------|-------------------------------------------------------------------------------------|
| <input type="checkbox"/> GSM537760 | 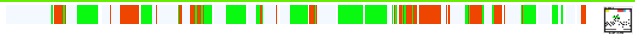 |
|------------------------------------|-------------------------------------------------------------------------------------|

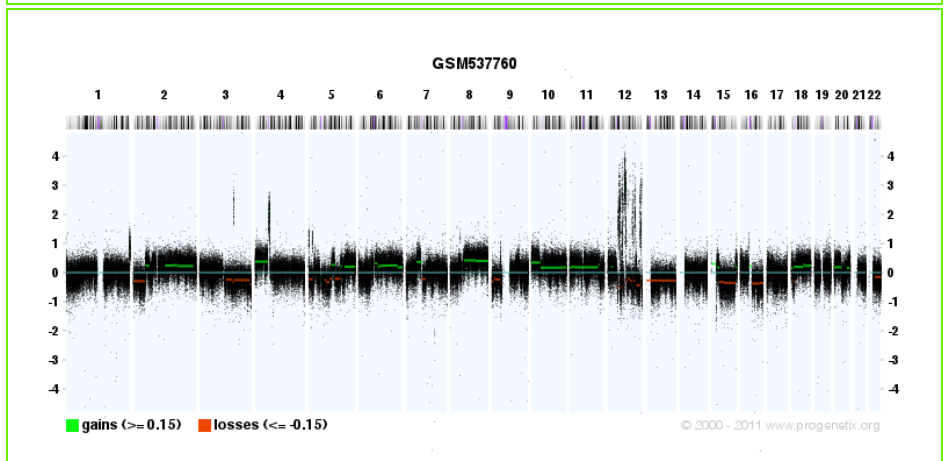

|                                    |                                                                                      |
|------------------------------------|--------------------------------------------------------------------------------------|
| ARRAYPLOT                          | <input type="button" value="PNG SVG"/>                                               |
| <input type="checkbox"/> GSM537761 | 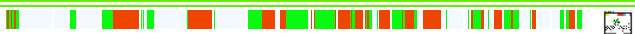 |

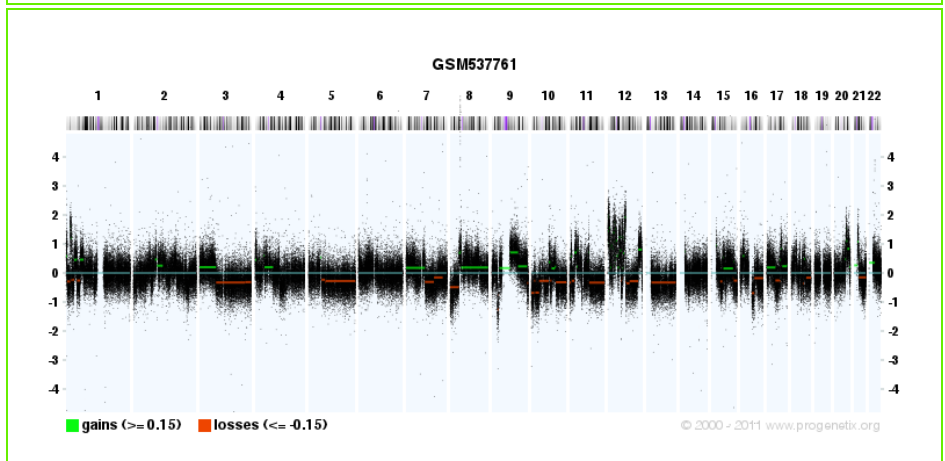

|           |                                        |
|-----------|----------------------------------------|
| ARRAYPLOT | <input type="button" value="PNG SVG"/> |
|-----------|----------------------------------------|

☐ GSM537762

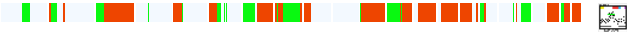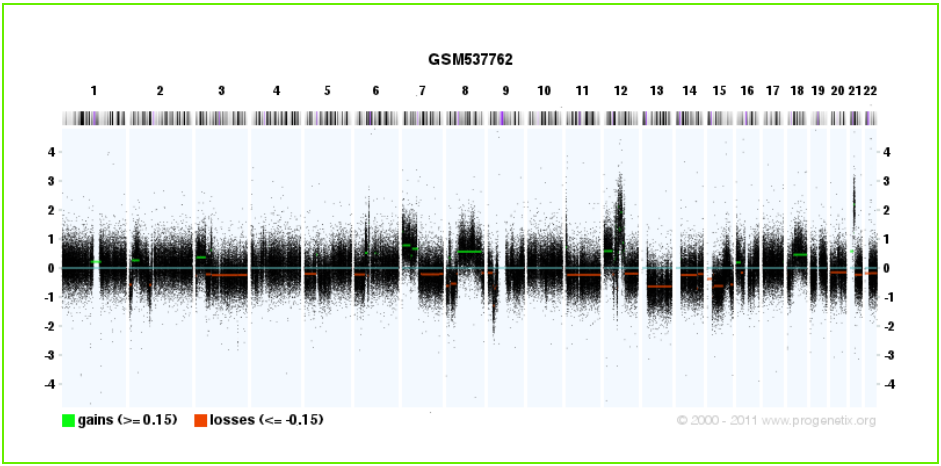

ARRAYPLOT

PNG SVG

☐ GSM537763

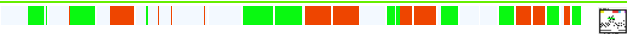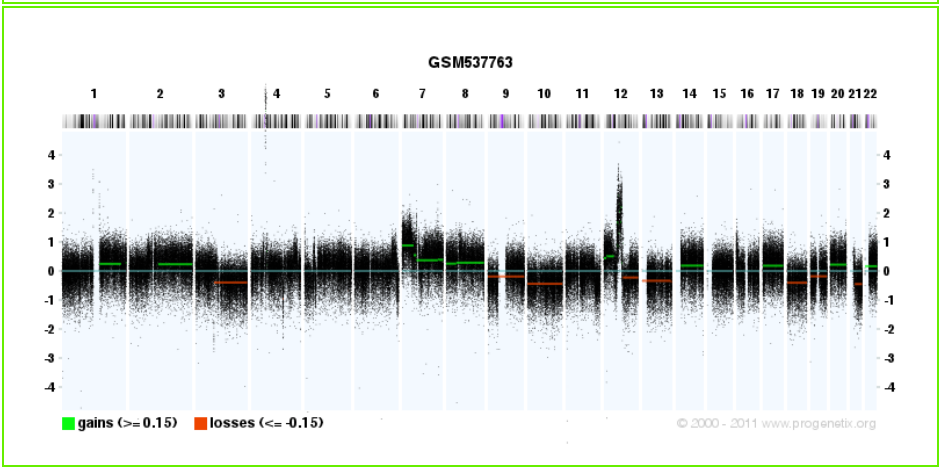

ARRAYPLOT

PNG SVG

☐ GSM537764

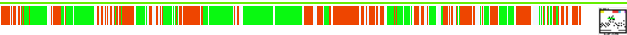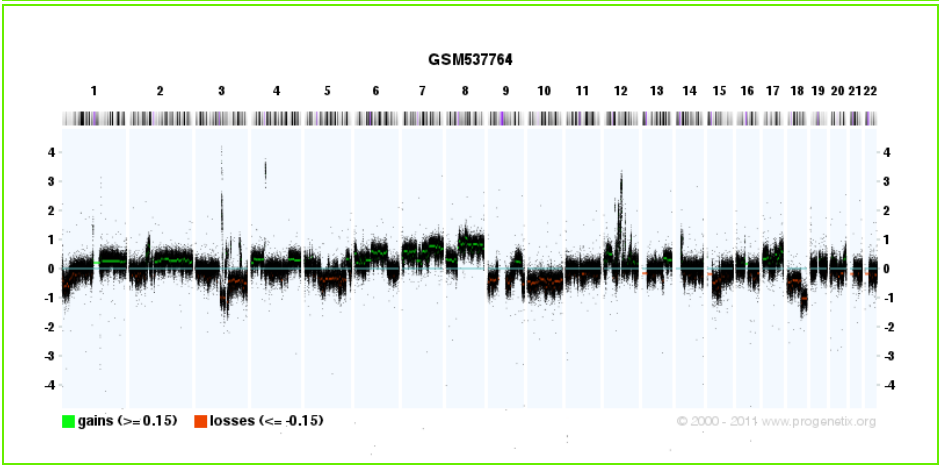

ARRAYPLOT

PNG SVG

☐ GSM537765

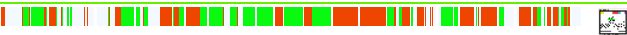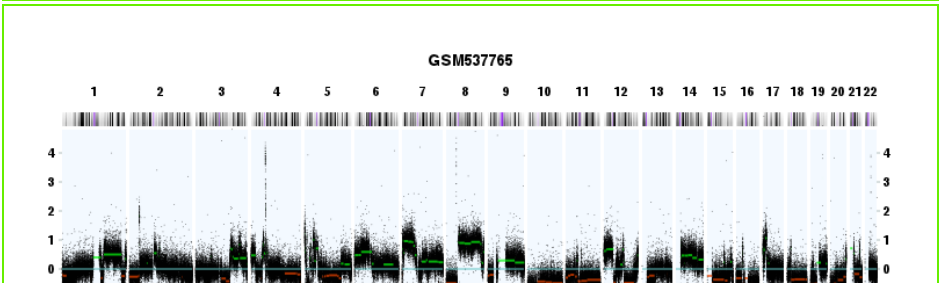

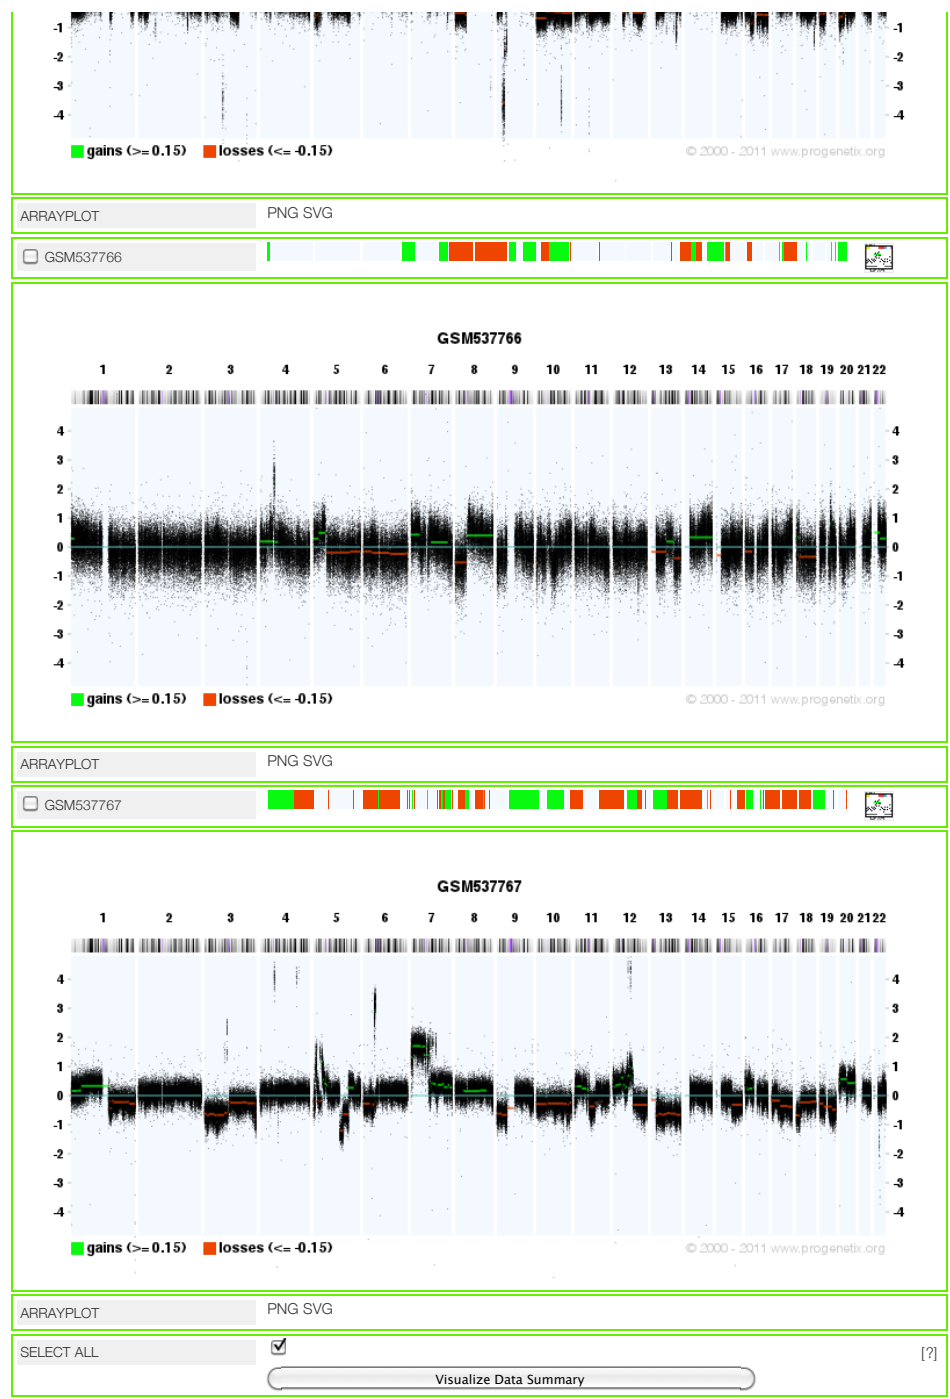

**Figure S1. Array data sets visualization.** Original plots and optimized parameters for GSE21530 which contains 8 intimal sarcoma samples hybridized on Agilent CGH Microarray 244A platform. The normalized probe signal log2 ratios and post-thresholding segmentation results for each array are intuitively displayed. Genomic alterations are represented by horizontal green (gain) and red (loss) lines. Alterations defined here as regions with log2 ratio 0.15 or -0.15. Simplified schemas of CNAs link to UCSC genome browser for further review.
