# Supplementary material for: arrayMap: A Reference Resource for Genomic Copy Number Imbalances in Human Malignancies
Source: arXiv:1201.2677 ancillary file (2012-01-11)
Supplement: Supplementary file 2 [file 20120111_Cai_Kumar_Baudis_arrayMap_supplement2.pdf]

[Search Public Series](#)[Search Public Arrays](#)[Plot Array Data](#)[Progenetix](#)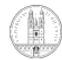University of  
Zurich <sup>uzh</sup>[News](#)[Citation](#)[FAQ & Guide](#)[Contributing Authors](#)[CompBio Zurich](#)[Atlas of Cytogenetics in  
Hematology/Oncology](#)[NCI SKY/M-FISH and  
CGH Database](#)[NCI Cancer Chromosomes](#)[FOLLOW US ON !\[\]\(4f6bf54ae7e4144a72d78316053e412d\_img.jpg\)](#)[Share](#) 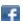 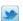 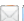 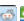 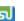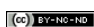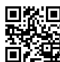

130.60.44.246

130.60.93.222

Visualization of genomic array data sets 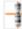 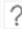

|                                                                                      |                                        |     |
|--------------------------------------------------------------------------------------|----------------------------------------|-----|
| SERIES                                                                               | <input type="text" value="GSE23452"/>  | [?] |
| ARRAY ID                                                                             | <input type="text" value="GSM630977"/> | [?] |
| <input type="button" value="Show original plots &amp; Load defaults (if existing)"/> |                                        |     |

|                      |                                              |                                     |               |                                  |     |
|----------------------|----------------------------------------------|-------------------------------------|---------------|----------------------------------|-----|
| CASE DATA PLOTTING   | <input type="text" value="no plot refresh"/> |                                     |               | [?]                              |     |
| GOLDEN PATH EDITION  | <input type="text" value="HG18 / 36"/>       |                                     |               | [?]                              |     |
| PLOT REGION          | <input type="text" value=""/>                |                                     |               | [?]                              |     |
| CHROMOSOMES TO PLOT  | <input type="text" value="1:22"/>            |                                     |               | [?]                              |     |
| LOSS/GAIN THRESHOLDS | <input type="text" value="-0.15"/>           | <input type="text" value="0.15"/>   | Y AXIS FACTOR | <input type="text" value="1.2"/> | [?] |
| REGION SIZE          | <input type="text" value="0"/>               | <input type="text" value="250000"/> | MIN. PROBES   | <input type="text" value="2"/>   | [?] |

|                                                           |                                                                                    |                                                     |     |
|-----------------------------------------------------------|------------------------------------------------------------------------------------|-----------------------------------------------------|-----|
| EMAIL / PASSWORD                                          | <input type="text" value="your registered email"/>                                 | <input type="text" value="your received password"/> | [?] |
| LICENSE AGREEMENT                                         | <input checked="" type="checkbox"/> I agree to license, disclaimer & citation note |                                                     |     |
| <input type="button" value="Filter / replot array data"/> |                                                                                    |                                                     |     |

|           |              |
|-----------|--------------|
| GSM630977 | 147 segments |
|-----------|--------------|

parsing database ...

|                    |                                                                    |                                                                                                                                                                                                                                                                                                                                                 |
|--------------------|--------------------------------------------------------------------|-------------------------------------------------------------------------------------------------------------------------------------------------------------------------------------------------------------------------------------------------------------------------------------------------------------------------------------------------|
| ARRAYID            | GSM630977                                                          | 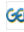 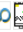 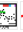 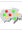 |
| PGCASEID           | GSM630977                                                          | 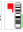                                                                                                                                                                                                                                                             |
| ARRAYNAME          | MIAML041T                                                          |                                                                                                                                                                                                                                                                                                                                                 |
| ARRAYDESCRIPTION   | primary human: blood or bone marrow, FACS sort-purified AML blasts |                                                                                                                                                                                                                                                                                                                                                 |
| DIAGNOSISTEXT      | Acute Myelogenous Leukemia                                         |                                                                                                                                                                                                                                                                                                                                                 |
| ICDMORPHOLOGY      | Acute myeloid leukemia, NOS                                        |                                                                                                                                                                                                                                                                                                                                                 |
| ICDMORPHOLOGYCODE  | 9861/3                                                             |                                                                                                                                                                                                                                                                                                                                                 |
| ICDOTOPOGRAPHY     | hematopoietic and reticuloendothelial systems                      |                                                                                                                                                                                                                                                                                                                                                 |
| ICDOTOPOGRAPHYCODE | C42                                                                |                                                                                                                                                                                                                                                                                                                                                 |
| PMID               | 20729466                                                           | 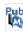 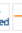 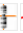                                                                                     |
| PLATFORMID         | GPL6801                                                            | 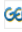                                                                                                                                                                                                                                                             |
| PLATFORMLABEL      | GenomeWideSNP_6                                                    |                                                                                                                                                                                                                                                                                                                                                 |
| PROBES             | 1880794                                                            |                                                                                                                                                                                                                                                                                                                                                 |
| QCVETO             | accept                                                             |                                                                                                                                                                                                                                                                                                                                                 |
| SERIESID           | GSE23452                                                           | 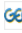                                                                                                                                                                                                                                                           |
| SAMPLESOURCE       | primary                                                            |                                                                                                                                                                                                                                                                                                                                                 |

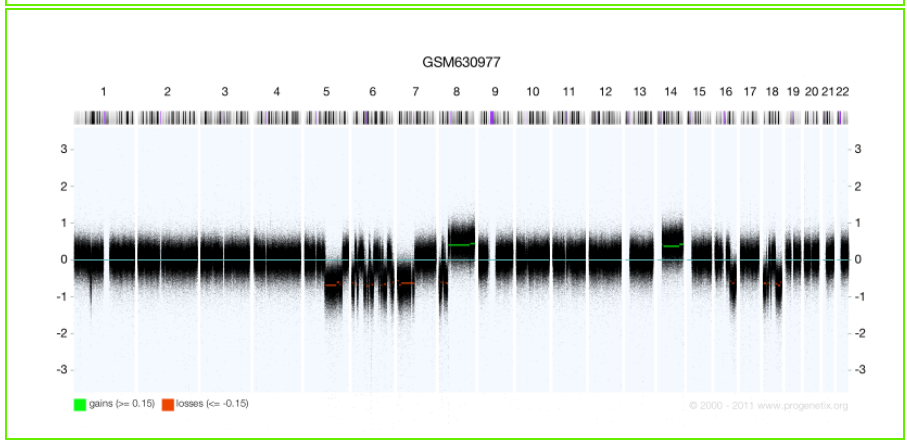

|           |     |
|-----------|-----|
| ARRAYPLOT | PNG |
|-----------|-----|

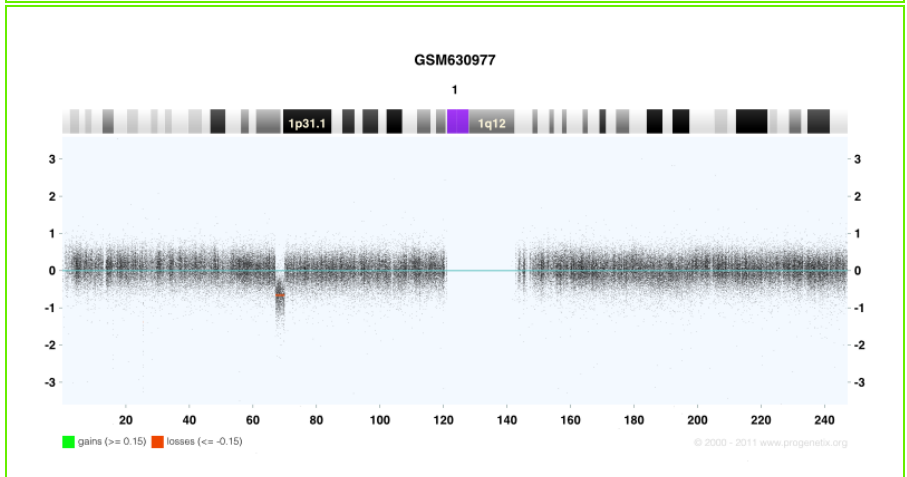

|                |         |
|----------------|---------|
| ARRAYPLOT,CHR1 | PNG SVG |
|----------------|---------|

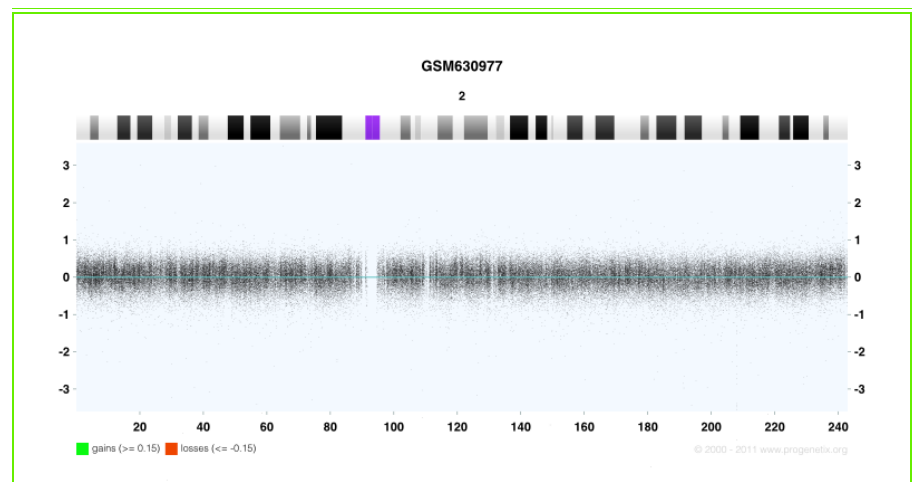

ARRAYPLOT,CHR2

PNG SVG

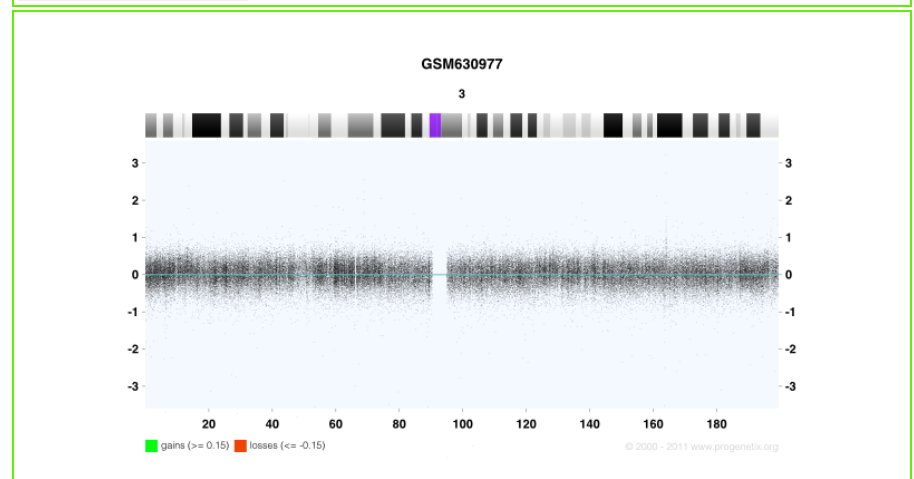

ARRAYPLOT,CHR3

PNG SVG

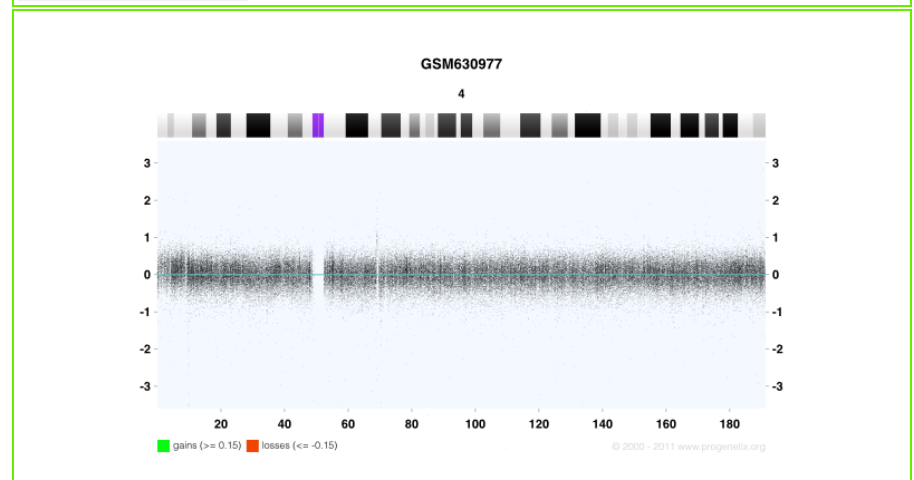

ARRAYPLOT,CHR4

PNG SVG

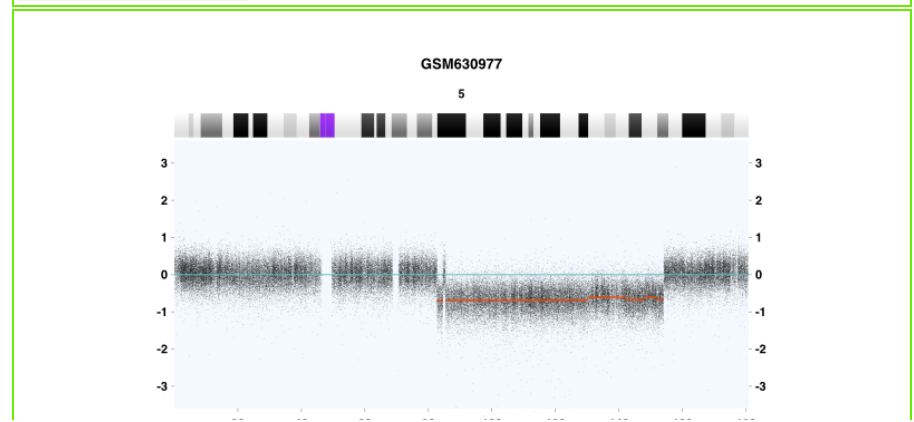

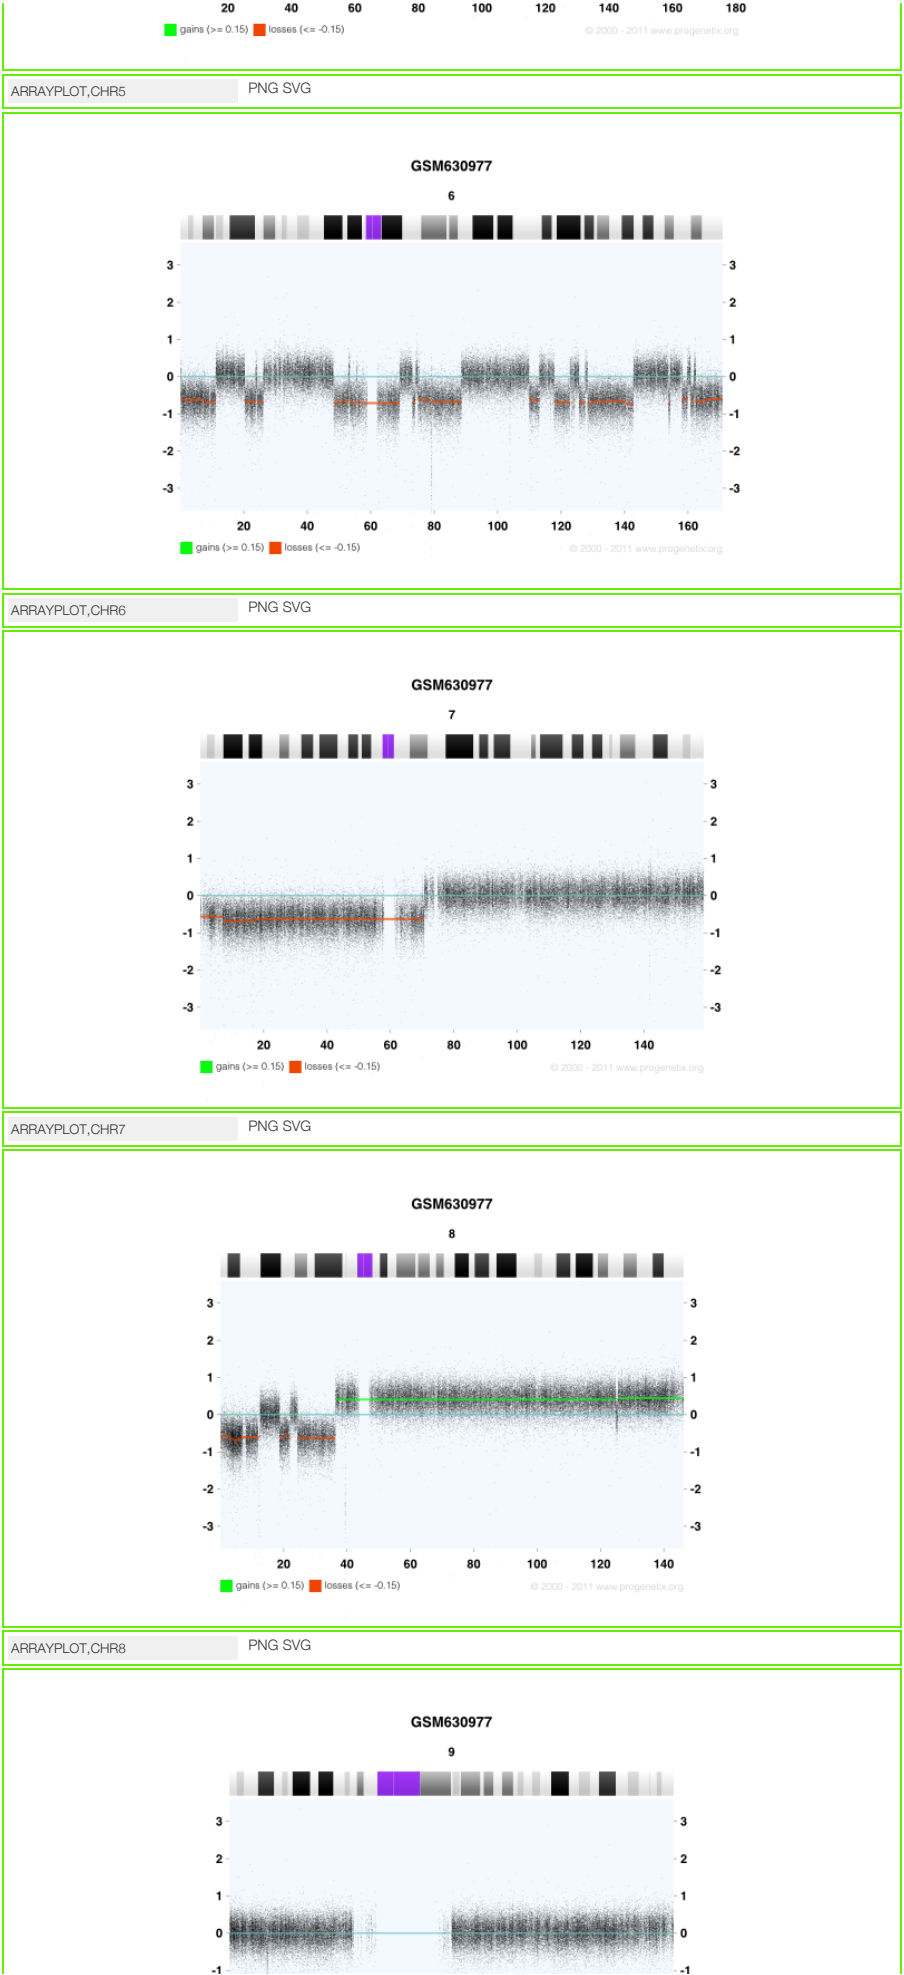

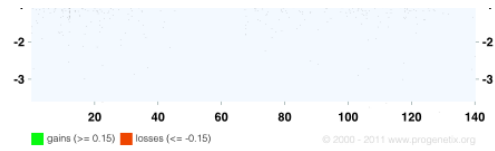

ARRAYPLOT,CHR9

PNG SVG

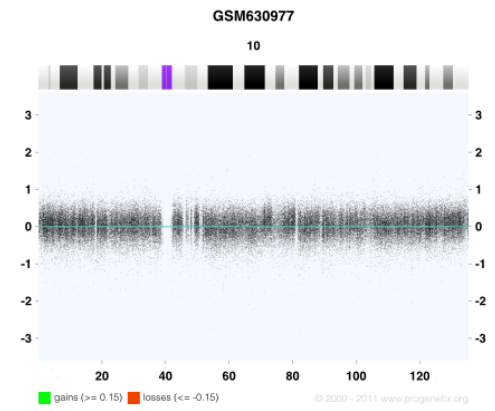

ARRAYPLOT,CHR10

PNG SVG

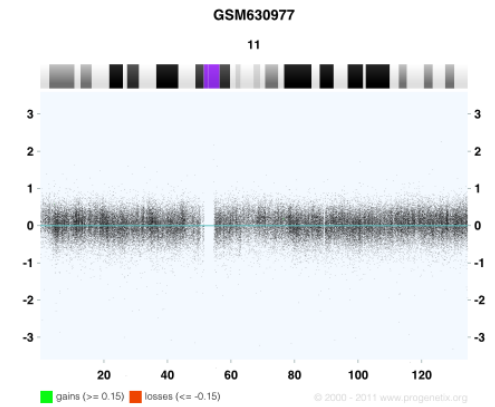

ARRAYPLOT,CHR11

PNG SVG

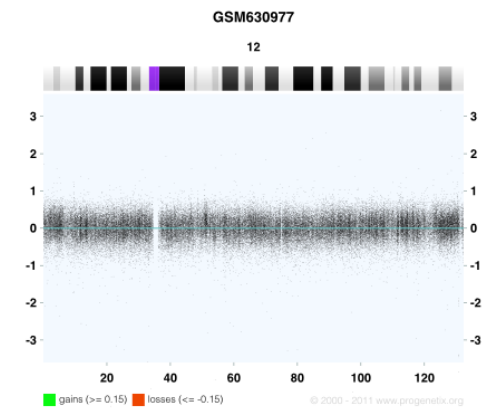

ARRAYPLOT,CHR12

PNG SVG

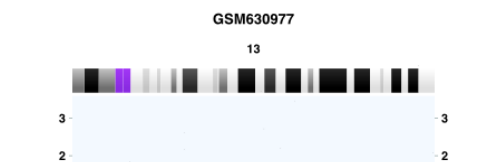

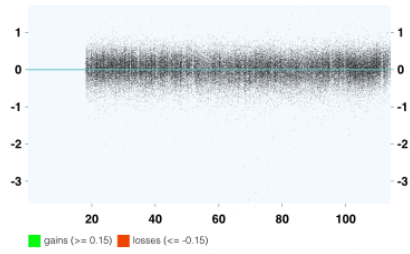

ARRAYPLOT,CHR13

PNG SVG

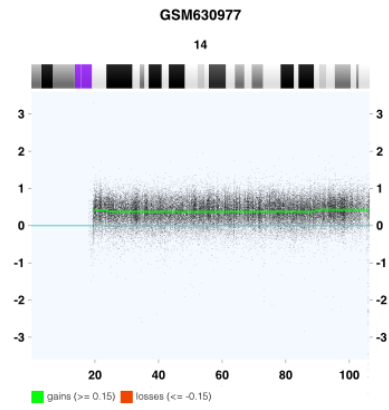

ARRAYPLOT,CHR14

PNG SVG

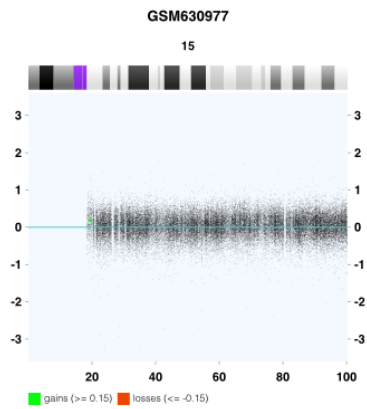

ARRAYPLOT,CHR15

PNG SVG

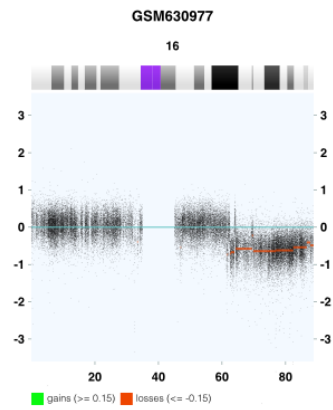

ARRAYPLOT,CHR16

PNG SVG

GSM630977

17

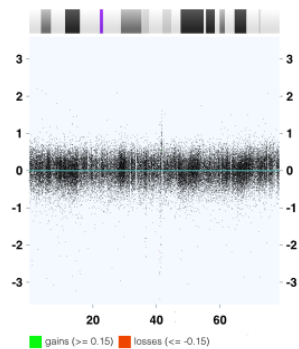

ARRAYPLOT,CHR17

PNG SVG

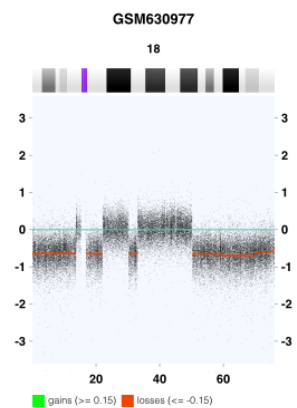

ARRAYPLOT,CHR18

PNG SVG

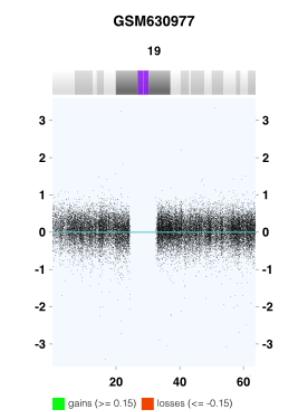

ARRAYPLOT,CHR19

PNG SVG

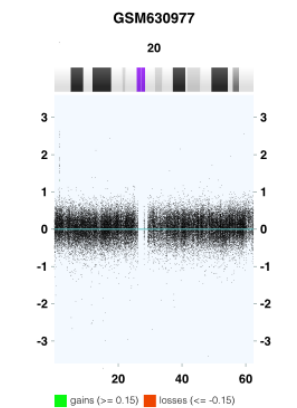

ARRAYPLOT,CHR20

PNG SVG

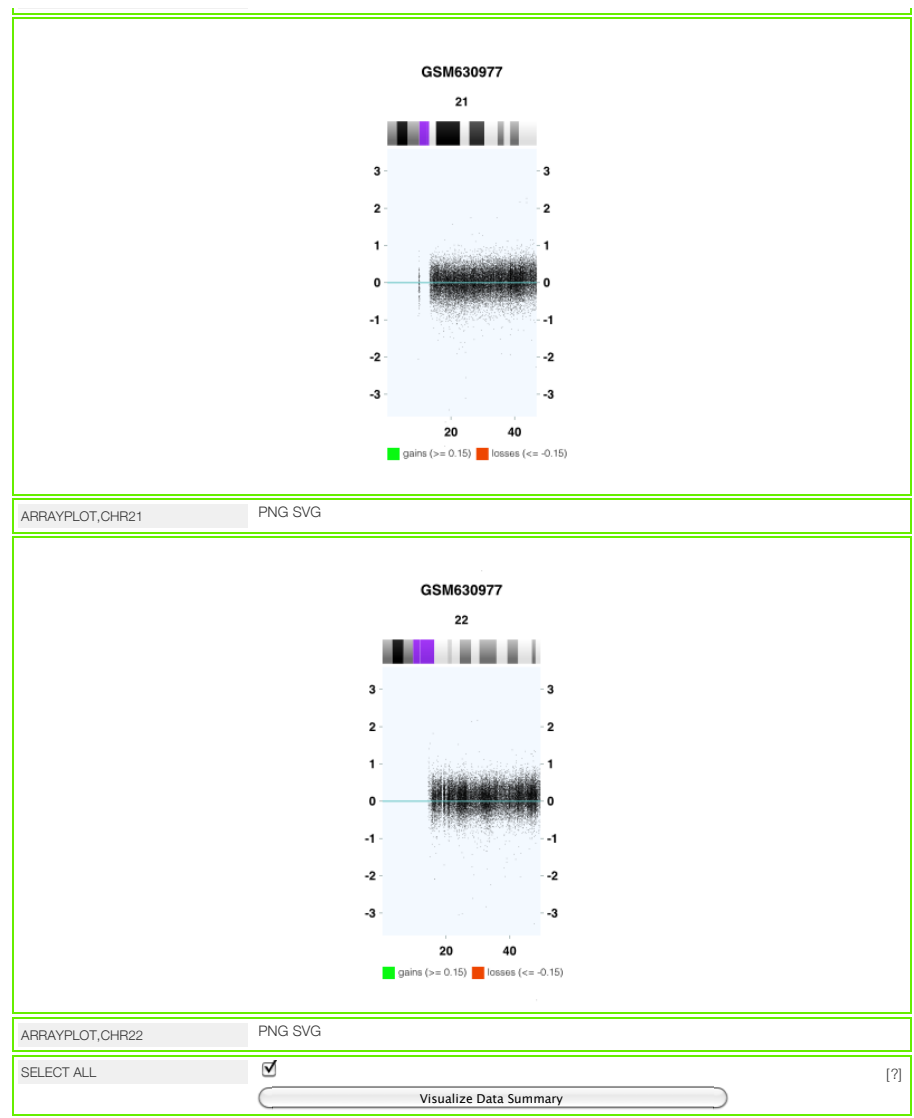

**Figure S2. Screenshot of single array visualization.** ArrayMap plots for GSM630977 (acute myelogenous leukemia). Besides the whole genome view, subviews of each chromosome are displayed as well. From these plots, different kinds of genetic variation events are clearly revealed, e.g. massive genomic rearrangement in chromosome 6; arm-level gain of chromosome 8q and 3MB focal change around 1p31.3. Through the "Plot Array Data" interface, users can segment the raw data values and re-plot the results with customized parameters.
