# Supplementary material for: arrayMap: A Reference Resource for Genomic Copy Number Imbalances in Human Malignancies
Source: arXiv:1201.2677 ancillary file (2012-01-11)
Supplement: Supplementary file 4 [file 20120111_Cai_Kumar_Baudis_arrayMap_supplement4.pdf]

Supplementary Table S1: Entities extracted from NCBI GEO and EBI ArrayExpress

| GSE ID   | GSM No | GPL ID                           | GPL No | Data Type     | Genome Version    | Array Type                                      |
|----------|--------|----------------------------------|--------|---------------|-------------------|-------------------------------------------------|
| GSE10007 | 4      | GPL2005                          | 1      | Affy CEL      | HG17              | In situ oligonucleotide                         |
| GSE10025 | 138    | GPL6317,GPL6318,GPL6319,GPL6320, | 7      | Log2          | Stanford IMAGE ID | spotted DNA/cDNA                                |
| GSE10060 | 2      | GPL2641                          | 1      | Affy CEL      | HG17              | In situ oligonucleotide                         |
| GSE10092 | 100    | GPL3718                          | 1      | Affy CEL      | HG17              | oligonucleotide                                 |
| GSE10099 | 626    | GPL2004,GPL2005                  | 2      | Affy CEL      | HG17              | oligonucleotide                                 |
| GSE10128 | 62     | GPL5772                          | 1      | Log2          | HG18              | BAC/P1                                          |
| GSE10129 | 56     | GPL5772                          | 1      | Log2          | HG18              | BAC/P1                                          |
| GSE10132 | 41     | GPL6359                          | 1      | Log2          |                   | spotted DNA/cDNA                                |
| GSE10179 | 42     | GPL6365                          | 1      | Log2          |                   | spotted DNA/cDNA                                |
| GSE10197 | 38     | GPL6382                          | 1      | Log2          | HG18              | spotted DNA/cDNA                                |
| GSE10266 | 5      | GPL5840                          | 1      | Log2          | HG17              | BAC/P1                                          |
| GSE10387 | 12     | GPL2005                          | 1      | Affy CEL      | HG17              | oligonucleotide                                 |
| GSE10423 | 6      | GPL6468                          | 1      | Log2          | Stanford IMAGE ID | spotted DNA/cDNA                                |
| GSE10456 | 15     | GPL6478                          | 1      | Log2          | HG18              | spotted DNA/cDNA                                |
| GSE10506 | 24     | GPL5711                          | 1      | LogR          | HG17              | spotted oligonucleotide                         |
| GSE10524 | 40     | GPL4012                          | 1      | Log2          | HG17              | spotted DNA/cDNA                                |
| GSE10583 | 20     | GPL2873                          | 1      | Log10         | HG17              | In situ oligonucleotide                         |
| GSE10600 | 29     | GPL6514                          | 1      | Log2          | HG18              | spotted DNA/cDNA                                |
| GSE10611 | 28     | GPL2004,GPL2005,GPL6520,GPL6521  | 4      | Affy CEL/Log2 | HG17              | BAC/P1                                          |
| GSE1065  | 14     | GPL1003                          | 1      | Log2          |                   | BAC/P1                                          |
| GSE1066  | 4      | GPL1005                          | 1      | Log2          |                   | BAC/P1                                          |
| GSE10747 | 35     | GPL1266,GPL3720                  | 2      | Affy CEL      | HG17/HG17         | In situ oligonucleotide/in situ oligonucleotide |
| GSE1078  | 19     | GPL1048                          | 1      | Log2          |                   | BAC/P1                                          |
| GSE10792 | 79     | GPL2004,GPL2005                  | 2      | Affy CEL      | HG17              | oligonucleotide                                 |
| GSE10822 | 13     | GPL6575                          | 1      | Log2          |                   | BAC/P1                                          |
| GSE10878 | 37     | GPL2879                          | 1      | Log2          | HG17              | In situ oligonucleotide                         |
| GSE10922 | 28     | GPL2005                          | 1      | Affy CEL      | HG17              | In situ oligonucleotide                         |
| GSE11036 | 12     | GPL2005                          | 1      | Affy CEL      | HG17              | In situ oligonucleotide                         |
| GSE11109 | 20     | GPL2879                          | 1      | Log10         | HG17              | In situ oligonucleotide                         |
| GSE11155 | 89     | GPL6737                          | 1      | Log2          | HG17              | BAC/P1                                          |
| GSE11225 | 4      | GPL2873,GPL6745                  | 2      | Log10/Log2    | HG17              | In situ oligonucleotide                         |

## GEO

|          |                             |            |                       |                                                         |
|----------|-----------------------------|------------|-----------------------|---------------------------------------------------------|
| GSE11263 | 44 GPL6782                  | 1 Log2     | HG17                  | BAC/P1                                                  |
| GSE11265 | 44 GPL6783                  | 1 Log2     | HG17                  | BAC/P1                                                  |
| GSE11275 | 86 GPL2043,GPL2616          | 2 Log2     | HG17/HG15             | BAC/P1                                                  |
| GSE11318 | 203 GPL6400                 | 1 Log2     | HG17                  | in situ oligonucleotide                                 |
| GSE11411 | 2 GPL4091                   | 1 Log10    | HG17                  | in situ oligonucleotide                                 |
| GSE11417 | 188 GPL2005                 | 1 Affy CEL | HG17                  | oligonucleotide                                         |
| GSE11447 | 75 GPL2641                  | 1 Affy CEL | HG17                  | in situ oligonucleotide                                 |
| GSE11573 | 52 GPL2843,GPL5477          | 2 Log2     | HG16/HG17             | BAC/P1/in situ oligonucleotide                          |
| GSE11782 | 10 GPL2641                  | 1 Affy CEL | HG17                  | in situ oligonucleotide                                 |
| GSE11872 | 8 GPL6853                   | 1 Log2     | HG18                  | BAC/P1                                                  |
| GSE11929 | 39 GPL2843,GPL3441          | 2 Log2     | HG16                  | BAC/P1                                                  |
| GSE11931 | 24 GPL3441                  | 1 Log2     | HG16                  | BAC/P1                                                  |
| GSE11938 | 10 GPL4091                  | 1 Log2     | HG17                  | in situ oligonucleotide                                 |
| GSE11945 | 29 GPL2616                  | 1 Log2     | HG15                  | BAC/P1                                                  |
| GSE11948 | 174 GPL3718,GPL3720         | 2 Affy CEL | HG17                  | in situ oligonucleotide                                 |
| GSE11960 | 114 GPL3718,GPL3720         | 2 Affy CEL | HG17                  | in situ oligonucleotide                                 |
| GSE11976 | 20 GPL6986                  | 1 LogR     | HG18                  | oligonucleotide                                         |
| GSE11977 | 6 GPL6981                   | 1 LogR     | HG18                  | oligonucleotide beads                                   |
| GSE12019 | 225 GPL3720                 | 1 Affy CEL | HG17                  | in situ oligonucleotide                                 |
| GSE12040 | 28 GPL4896                  | 1 Log2     |                       | BAC/P1                                                  |
| GSE12225 | 35 GPL2641                  | 1 Affy CEL | HG17                  | in situ oligonucleotide                                 |
| GSE12280 | 34 GPL7096                  | 1 Log      |                       | BAC/P1                                                  |
| GSE12393 | 106 GPL2616                 | 1 Log2     | HG15                  | BAC/P1                                                  |
| GSE12439 | 67 GPL4723,GPL7203          | 2 Log2     | HG17                  | BAC/P1/in situ oligonucleotide                          |
| GSE12461 | 1 GPL2004                   | 1 Affy CEL | HG17                  | oligonucleotide                                         |
| GSE12494 | 262 GPL2004,GPL2005,GPL3718 | 3 Affy CEL | HG17                  | oligonucleotide/oligonucleotide/in situ oligonucleotide |
| GSE12520 | 139 GPL7199,GPL9336         | 2 Log2     | HG17/Ensembl 22.34d.1 | spotted DNA/cDNA                                        |
| GSE12523 | 31 GPL6853                  | 1 Log2     | HG18                  | BAC/P1                                                  |
| GSE12593 | 4 GPL4723                   | 1 Log2     | HG17                  | BAC/P1                                                  |
| GSE12659 | 16 GPL2879                  | 1 Log2     | HG17                  | in situ oligonucleotide                                 |
| GSE12660 | 25 GPL3718                  | 1 Affy CEL | HG17                  | in situ oligonucleotide                                 |
| GSE12668 | 42 GPL4091                  | 1 Log2     | HG17                  | in situ oligonucleotide                                 |
| GSE12702 | 80 GPL3718,GPL3720          | 2 Affy CEL | HG17                  | in situ oligonucleotide                                 |
| GSE12759 | 56 GPL4723,GPL7247          | 2 Log2     | HG17/HG17             | BAC/P1                                                  |

## GEO

|          |                                      |                 |                   |                                                         |
|----------|--------------------------------------|-----------------|-------------------|---------------------------------------------------------|
| GSE12761 | 72 GPL7298                           | 1 Log2          | HG16              | BAC/P1                                                  |
| GSE12794 | 168 GPL7313,GPL7314                  | 2 Log2          | HG18              | in situ oligonucleotide                                 |
| GSE12808 | 19 GPL2641,GPL3718                   | 2 Affy CEL      | HG17              | in situ oligonucleotide                                 |
| GSE12813 | 172 GPL6322,GPL7321,GPL7322,GPL7323, | 6 Log2          | Stanford IMAGE ID | spotted DNA/cDNA                                        |
| GSE12830 | 20 GPL4091,GPL4544                   | 2 Log10         | HG17/HG17         | in situ oligonucleotide                                 |
| GSE12896 | 384 GPL3718,GPL3720                  | 2 Affy CEL      | HG17              | in situ oligonucleotide                                 |
| GSE12902 | 22 GPL4012                           | 1 Log2          | HG17              | spotted DNA/cDNA                                        |
| GSE12906 | 332 GPL2004,GPL2005,GPL3718,GPL3720  | 4 Affy CEL      | HG17              | oligonucleotide/in situ oligonucleotide                 |
| GSE12928 | 2 GPL5477                            | 1 Log2          | HG17              | in situ oligonucleotide                                 |
| GSE12951 | 28 GPL2843,GPL5477,GPL7394           | 3 Log2          | HG16/HG17/HG17    | BAC/P1/in situ oligonucleotide/BAC/P1                   |
| GSE12958 | 2 GPL5477                            | 1 Log2          | HG17              | in situ oligonucleotide                                 |
| GSE13021 | 58 GPL3718                           | 1 Affy CEL      | HG17              | in situ oligonucleotide                                 |
| GSE13137 | 23 GPL2004                           | 1 Affy CEL      | HG17              | oligonucleotide                                         |
| GSE13191 | 30 GPL2819,GPL3055                   | 2 Log2          | HG17/HG17         | spotted oligonucleotide                                 |
| GSE13239 | 25 GPL2879                           | 1 Log           | HG17              | in situ oligonucleotide                                 |
| GSE13282 | 21 GPL6982                           | 1 LogR          | HG18              | oligonucleotide beads                                   |
| GSE13331 | 54 GPL2616,GPL4544                   | 2 Log2/Log10    | HG15/HG17         | BAC/P1/in situ oligonucleotide                          |
| GSE13372 | 68 GPL6801                           | 1 Affy CEL      | HG18              | in situ oligonucleotide                                 |
| GSE13429 | 49 GPL3718,GPL6801                   | 2 Affy CEL      | HG17/HG18         | in situ oligonucleotide/in situ oligonucleotide         |
| GSE13439 | 4 GPL3718                            | 1 Affy CEL      | HG17              | in situ oligonucleotide                                 |
| GSE13557 | 40 GPL3718,GPL4723,GPL5149,GPL6980   | 3 Affy CEL/Log2 | HG17/HG17/HG18    | BAC/P1/spotted oligonucleotide/oligonucleotide          |
| GSE13612 | 23 GPL3718                           | 1 Affy CEL      | HG17              | in situ oligonucleotide                                 |
| GSE13696 | 90 GPL2004,GPL2005                   | 2 Affy CEL      | HG17              | oligonucleotide                                         |
| GSE13775 | 49 GPL4723                           | 1 Log2          | HG17              | BAC/P1                                                  |
| GSE13813 | 118 GPL2005                          | 1 Affy CEL      | HG17              | oligonucleotide                                         |
| GSE13914 | 55 GPL7778,GPL7779,GPL7780,GPL7781,  | 7 Log2          | Stanford IMAGE ID | spotted DNA/cDNA                                        |
| GSE13989 | 27 GPL3718                           | 1 Affy CEL      | HG17              | in situ oligonucleotide                                 |
| GSE14016 | 54 GPL2005,GPL3718                   | 2 Affy CEL      | HG17              | oligonucleotide/in situ oligonucleotide                 |
| GSE14079 | 8 GPL1998                            | 1 Log2          | Stanford IMAGE ID | spotted DNA/cDNA                                        |
| GSE14087 | 134 GPL3718,GPL3720                  | 2 Affy CEL      | HG17              | in situ oligonucleotide                                 |
| GSE14109 | 33 GPL2873,GPL7823                   | 2 Log2          | HG17              | in situ oligonucleotide                                 |
| GSE14248 | 2 GPL3718                            | 1 Affy CEL      | HG17              | in situ oligonucleotide                                 |
| GSE14353 | 17 GPL8036                           | 1 Copy Number   |                   | in situ oligonucleotide                                 |
| GSE14437 | 424 GPL2004,GPL2005,GPL3718          | 3 Affy CEL      | HG17              | oligonucleotide/oligonucleotide/in situ oligonucleotide |

## GEO

|          |                             |               |           |                                                         |
|----------|-----------------------------|---------------|-----------|---------------------------------------------------------|
| GSE14579 | 40 GPL2004,GPL2005          | 2 Affy CEL    |           | in situ oligonucleotide                                 |
| GSE14582 | 181 GPL2641                 | 1 Affy CEL    | HG17      | in situ oligonucleotide                                 |
| GSE14656 | 54 GPL2004,GPL2005          | 2 Affy CEL    | HG17      | oligonucleotide                                         |
| GSE14670 | 120 GPL2641,GPL3718         | 2 Affy CEL    | HG17      | in situ oligonucleotide                                 |
| GSE14740 | 24 GPL8036                  | 1 Copy Number |           | in situ oligonucleotide                                 |
| GSE14741 | 46 GPL8036                  | 1 Copy Number |           | in situ oligonucleotide                                 |
| GSE14742 | 50 GPL8036                  | 1 Copy Number |           | in situ oligonucleotide                                 |
| GSE14743 | 12 GPL8036                  | 1 Copy Number |           | in situ oligonucleotide                                 |
| GSE14744 | 56 GPL8036                  | 1 Copy Number |           | in situ oligonucleotide                                 |
| GSE14745 | 38 GPL8036                  | 1 Copy Number |           | in situ oligonucleotide                                 |
| GSE14803 | 15 GPL5114                  | 1 Log2        | HG17      | BAC/P1                                                  |
| GSE14804 | 21 GPL2005                  | 1 Affy CEL    | HG17      | oligonucleotide                                         |
| GSE14819 | 23 GPL8175                  | 1 Log2        |           | BAC/P1                                                  |
| GSE14820 | 8 GPL8175                   | 1 Log2        |           | BAC/P1                                                  |
| GSE14821 | 4 GPL8175                   | 1 Log2        |           | BAC/P1                                                  |
| GSE14822 | 20 GPL8175                  | 1 Log2        |           | BAC/P1                                                  |
| GSE14823 | 7 GPL8175                   | 1 Log2        |           | BAC/P1                                                  |
| GSE14859 | 26 GPL8186                  | 1 Log2        | HG16      | BAC/P1                                                  |
| GSE14860 | 234 GPL2004,GPL2005         | 2 Affy CEL    | HG17      | oligonucleotide                                         |
| GSE14867 | 4 GPL6801                   | 1 Affy CEL    | HG18      | in situ oligonucleotide                                 |
| GSE14959 | 40 GPL4091                  | 1 Log2        | HG17      | in situ oligonucleotide                                 |
| GSE14960 | 23 GPL3718                  | 1 Affy CEL    | HG17      | oligonucleotide                                         |
| GSE14994 | 159 GPL3720                 | 1 Affy CEL    | HG17      | in situ oligonucleotide                                 |
| GSE14996 | 74 GPL8226                  | 1 Copy Number | HG18      | in situ oligonucleotide                                 |
| GSE15027 | 5 GPL8233                   | 1 Log2        | HG18      | in situ oligonucleotide                                 |
| GSE15051 | 6 GPL3720                   | 1 Affy CEL    | HG17      | in situ oligonucleotide                                 |
| GSE15079 | 5 GPL8187                   | 1 Log2        | HG16      | BAC/P1                                                  |
| GSE15126 | 20 GPL3718,GPL6801          | 2 Affy CEL    | HG17/HG18 | in situ oligonucleotide/in situ oligonucleotide         |
| GSE15127 | 12 GPL3718                  | 1 Affy CEL    | HG17      | oligonucleotide                                         |
| GSE15130 | 35 GPL4091                  | 1 Log10       | HG17      | in situ oligonucleotide                                 |
| GSE15131 | 13 GPL4091                  | 1 Log10       | HG17      | in situ oligonucleotide                                 |
| GSE15172 | 4 GPL4091                   | 1 Log10       | HG17      | in situ oligonucleotide                                 |
| GSE15177 | 77 GPL8276                  | 1 Log2        | HG17      | spotted oligonucleotide                                 |
| GSE15187 | 171 GPL2004,GPL2005,GPL3718 | 3 Affy CEL    | HG17      | oligonucleotide/oligonucleotide/in situ oligonucleotide |

## GEO

|          |                                     |                 |                   |                         |
|----------|-------------------------------------|-----------------|-------------------|-------------------------|
| GSE15264 | 3 GPL6801                           | 1 Affy CEL      | HG18              | in situ oligonucleotide |
| GSE15436 | 56 GPL5772                          | 1 Log2          | HG18              | BAC/P1                  |
| GSE15470 | 48 GPL8368                          | 1 Log2          | HG17              | spotted oligonucleotide |
| GSE15477 | 6 GPL8355                           | 1 Log10         |                   | in situ oligonucleotide |
| GSE15521 | 5 GPL5571                           | 1 Log2          | HG17              | in situ oligonucleotide |
| GSE15526 | 264 GPL3718,GPL3720                 | 2 Affy CEL      | HG17              | in situ oligonucleotide |
| GSE15688 | 122 GPL3718,GPL6801                 | 2 Affy CEL      | HG17/HG18         | in situ oligonucleotide |
| GSE15695 | 336 GPL3718,GPL3720                 | 2 Affy CEL      | HG17              | in situ oligonucleotide |
| GSE15696 | 27 GPL2004,GPL3718                  | 2 Affy CEL      | HG17              | oligonucleotide         |
| GSE15714 | 175 GPL2004                         | 1 Affy CEL      | HG17              | oligonucleotide         |
| GSE15730 | 176 GPL2004                         | 1 Affy CEL      | HG17              | oligonucleotide         |
| GSE15731 | 176 GPL2004                         | 1 Affy CEL      | HG17              | oligonucleotide         |
| GSE15732 | 175 GPL2004                         | 1 Affy CEL      | HG17              | oligonucleotide         |
| GSE15842 | 67 GPL3720                          | 1 Affy CEL      | HG17              | in situ oligonucleotide |
| GSE15931 | 27 GPL3720                          | 1 Affy CEL      | HG17              | in situ oligonucleotide |
| GSE16    | 25 GPL28                            | 1 Log2          |                   | BAC/P1                  |
| GSE16019 | 80 GPL6979,GPL6980                  | 2 LogR          | HG17/HG18         | oligonucleotide beads   |
| GSE16041 | 27 GPL6088                          | 1 Log2          | HG17              | spotted DNA/cDNA        |
| GSE16092 | 50 GPL3718                          | 1 Affy CEL      | HG17              | in situ oligonucleotide |
| GSE16121 | 45 GPL2005                          | 1 Affy CEL      | HG17              | oligonucleotide         |
| GSE16125 | 48 GPL3718                          | 1 Affy CEL      | HG17              | in situ oligonucleotide |
| GSE16384 | 20 GPL8634                          | 1 Log2          | HG17              | BAC/P1                  |
| GSE16400 | 179 GPL9704,GPL4091,GPL6986,GPL9708 | 4 Affy CEL/Log2 |                   |                         |
| GSE16406 | 203 GPL3718                         | 1 Affy CEL      | HG17              | oligonucleotide         |
| GSE16408 | 51 GPL8641                          | 1 Log2          | Stanford IMAGE ID | spotted DNA/cDNA        |
| GSE16511 | 47 GPL4560                          | 1 Log2          |                   | BAC/P1                  |
| GSE16575 | 2 GPL8693                           | 1 Log2          |                   | in situ oligonucleotide |
| GSE16597 | 36 GPL8690                          | 1 Log2          | HG18              | BAC/P1                  |
| GSE16598 | 4 GPL8581                           | 1 Log2          | HG17              | in situ oligonucleotide |
| GSE16599 | 4 GPL8581                           | 1 Log2          | HG17              | in situ oligonucleotide |
| GSE16600 | 4 GPL8581                           | 1 Log2          | HG17              | in situ oligonucleotide |
| GSE16601 | 4 GPL8581                           | 1 Log2          | HG17              | in situ oligonucleotide |
| GSE16602 | 6 GPL8581                           | 1 Log2          | HG17              | in situ oligonucleotide |
| GSE16603 | 5 GPL8581                           | 1 Log2          | HG17              | in situ oligonucleotide |

## GEO

|          |                             |                         |                   |                                                 |
|----------|-----------------------------|-------------------------|-------------------|-------------------------------------------------|
| GSE16604 | 4 GPL8581                   | 1 Log2                  | HG17              | in situ oligonucleotide                         |
| GSE16605 | 5 GPL8581                   | 1 Log2                  | HG17              | in situ oligonucleotide                         |
| GSE16606 | 7 GPL8581                   | 1 Log2                  | HG17              | in situ oligonucleotide                         |
| GSE16607 | 14 GPL8581                  | 1 Log2                  | HG17              | in situ oligonucleotide                         |
| GSE16608 | 6 GPL8581                   | 1 Log2                  | HG17              | in situ oligonucleotide                         |
| GSE16609 | 9 GPL8581                   | 1 Log2                  | HG17              | in situ oligonucleotide                         |
| GSE16610 | 7 GPL8581                   | 1 Log2                  | HG17              | in situ oligonucleotide                         |
| GSE16611 | 8 GPL8581                   | 1 Log2                  | HG17              | in situ oligonucleotide                         |
| GSE16619 | 203 GPL3718,GPL3720,GPL6804 | 3 Affy CEL              | HG17/HG17/HG18    | in situ oligonucleotide                         |
| GSE16663 | 4 GPL8720                   | 1 Log2                  | HG17              | in situ oligonucleotide                         |
| GSE16664 | 4 GPL8720                   | 1 Log2                  | HG17              | in situ oligonucleotide                         |
| GSE16665 | 7 GPL8720                   | 1 Log2                  | HG17              | in situ oligonucleotide                         |
| GSE16667 | 4 GPL8720                   | 1 Log2                  | HG17              | in situ oligonucleotide                         |
| GSE16668 | 7 GPL8720                   | 1 Log2                  | HG17              | in situ oligonucleotide                         |
| GSE16669 | 4 GPL8720                   | 1 Log2                  | HG17              | in situ oligonucleotide                         |
| GSE16680 | 97 GPL4560                  | 1 Log2                  | BAC/P1            |                                                 |
| GSE16718 | 104 GPL6804                 | 1 Affy CEL              | HG18              | in situ oligonucleotide                         |
| GSE16724 | 2 GPL8737                   | 1 Log2                  | HG18              | in situ oligonucleotide                         |
| GSE16746 | 100 GPL3718                 | 1 Affy CEL              | HG17              | in situ oligonucleotide                         |
| GSE16872 | 6 GPL8774                   | 1 Log2                  | HG15              | spotted DNA/cDNA                                |
| GSE16937 | 21 GPL2641                  | 1 Affy CEL              | HG17              | in situ oligonucleotide                         |
| GSE17047 | 42 GPL8693,GPL8841,GPL10197 | 3 Log2/Signal Intensity | HG18/HG17/HG18    | in situ oligonucleotide                         |
| GSE1715  | 29 GPL1424                  | 1 Log2                  |                   | spotted DNA/cDNA                                |
| GSE17165 | 16 GPL4091,GPL8876          | 2 Log10                 | HG17              | in situ oligonucleotide/spotted oligonucleotide |
| GSE17181 | 40 GPL8841                  | 1 Log2                  | HG17              | in situ oligonucleotide                         |
| GSE17247 | 84 GPL3720                  | 1 Affy CEL              | HG17              | in situ oligonucleotide                         |
| GSE17359 | 18 GPL6801                  | 1 Affy CEL              | HG18              | in situ oligonucleotide                         |
| GSE17381 | 24 GPL4091                  | 1 Log10                 | HG17              | in situ oligonucleotide                         |
| GSE17396 | 11 GPL4093                  | 1 Log10                 | HG17              | in situ oligonucleotide                         |
| GSE17429 | 30 GPL3720                  | 1 Affy CEL              | HG17              | in situ oligonucleotide                         |
| GSE17498 | 19 GPL2005                  | 1 Affy CEL              | HG17              | oligonucleotide                                 |
| GSE17534 | 104 GPL3720                 | 1 Affy CEL              | HG17              | in situ oligonucleotide                         |
| GSE1755  | 8 GPL1448                   | 1 Log2                  | Stanford IMAGE ID | spotted DNA/cDNA                                |
| GSE17555 | 24 GPL8999                  | 1 Log10                 | Stanford IMAGE ID | spotted DNA/cDNA                                |

## GEO

|          |                             |            |           |                                                         |
|----------|-----------------------------|------------|-----------|---------------------------------------------------------|
| GSE17595 | 56 GPL1266,GPL2641          | 2 Affy CEL | HG17      | in situ oligonucleotide                                 |
| GSE17668 | 20 GPL9041,GPL9042          | 2 Log2     | HG18      | in situ oligonucleotide                                 |
| GSE17715 | 1 GPL8687                   | 1 Log2     | HG18      | in situ oligonucleotide                                 |
| GSE17907 | 54 GPL9128                  | 1 Log2     | HG17      | in situ oligonucleotide                                 |
| GSE17958 | 87 GPL3720                  | 1 Affy CEL | HG17      | in situ oligonucleotide                                 |
| GSE18098 | 41 GPL2879,GPL7823          | 2 Log2     | HG17      | in situ oligonucleotide                                 |
| GSE18143 | 2 GPL9202                   | 1 Log10    |           | in situ oligonucleotide                                 |
| GSE18154 | 42 GPL9216                  | 2 Log2     |           | spotted oligonucleotide                                 |
| GSE18166 | 131 GPL9189                 | 1 Log2     |           | spotted DNA/cDNA                                        |
| GSE18187 | 21 GPL5114                  | 1 Log2     | HG17      | BAC/P1                                                  |
| GSE18197 | 212 GPL3718,GPL3720         | 2 Affy CEL | HG17      | in situ oligonucleotide                                 |
| GSE18252 | 162 GPL2004,GPL2005         | 2 Affy CEL | HG17      | oligonucleotide                                         |
| GSE18259 | 54 GPL6737                  | 1 Log2     | HG17      | BAC/P1                                                  |
| GSE18333 | 82 GPL6801                  | 1 Affy CEL | HG18      | in situ oligonucleotide                                 |
| GSE18408 | 16 GPL4091                  | 1 Log10    | HG17      | in situ oligonucleotide                                 |
| GSE18453 | 105 GPL2879                 | 1 Log2     | HG17      | in situ oligonucleotide                                 |
| GSE18461 | 7 GPL6984                   | 1 LogR     | HG18      | oligonucleotide beads                                   |
| GSE18626 | 106 GPL4560                 | 1 Log2     |           | BAC/P1                                                  |
| GSE18638 | 98 GPL9128                  | 1 Log2     | HG17      | in situ oligonucleotide                                 |
| GSE18797 | 12 GPL3720                  | 1 Affy CEL | HG17      | in situ oligonucleotide                                 |
| GSE18799 | 21 GPL6980                  | 1 LogR     | HG18      | oligonucleotide beads                                   |
| GSE18820 | 34 GPL3718                  | 1 Affy CEL | HG17      | oligonucleotide                                         |
| GSE18828 | 18 GPL3718,GPL6801          | 2 Affy CEL | HG17/HG18 | in situ oligonucleotide/in situ oligonucleotide         |
| GSE18964 | 66 GPL3718                  | 1 Affy CEL | HG17      | oligonucleotide                                         |
| GSE19101 | 510 GPL2004,GPL2005,GPL3718 | 3 Affy CEL | HG17      | oligonucleotide/oligonucleotide/in situ oligonucleotide |
| GSE19159 | 168 GPL9715                 | 1 Log2     | HG18      | BAC/P1                                                  |
| GSE19177 | 34 GPL6986                  | 1 LogR     | HG18      | oligonucleotide                                         |
| GSE19180 | 10 GPL2879                  | 1 Log2     | HG17      | in situ oligonucleotide                                 |
| GSE19189 | 20 GPL6985                  | 1 LogR     | HG18      | oligonucleotide beads                                   |
| GSE19193 | 58 GPL4999                  | 1 Log2     |           | spotted DNA/cDNA                                        |
| GSE19318 | 1 GPL9944                   | 1 Log2     | HG18      | in situ oligonucleotide                                 |
| GSE19349 | 16 GPL8887                  | 1 LogR     |           | oligonucleotide beads                                   |
| GSE19388 | 13 GPL3720                  | 1 Affy CEL | HG17      | in situ oligonucleotide                                 |
| GSE19399 | 826 GPL3720                 | 1 Affy CEL | HG17      | in situ oligonucleotide                                 |

## GEO

|          |                            |                        |                   |                         |
|----------|----------------------------|------------------------|-------------------|-------------------------|
| GSE19416 | 7 GPL6801                  | 1 Affy CEL             | HG18              | in situ oligonucleotide |
| GSE19425 | 510 GPL9775,GPL9776        | 2 Log2                 | HG17              | in situ oligonucleotide |
| GSE19449 | 3 GPL2005                  | 1 Affy CEL             | HG17              | in situ oligonucleotide |
| GSE19458 | 11 GPL9797                 | 1 Log10                | HG16              | in situ oligonucleotide |
| GSE19459 | 20 GPL9798                 | 1 Log10                | HG17              | in situ oligonucleotide |
| GSE19523 | 12 GPL2004,GPL2005         | 2 Affy CEL             | HG17              | oligonucleotide         |
| GSE19539 | 72 GPL6801                 | 1 Affy CEL             | HG18              | in situ oligonucleotide |
| GSE19561 | 20 GPL9816                 | 1 Log2                 | HG17              | in situ oligonucleotide |
| GSE19566 | 20 GPL9128                 | 1 Log2                 | HG17              | in situ oligonucleotide |
| GSE19574 | 20 GPL9128                 | 1 Log2                 | HG17              | in situ oligonucleotide |
| GSE19578 | 156 GPL3718,GPL3720        | 2 Affy CEL             | HG17              | in situ oligonucleotide |
| GSE19594 | 88 GPL1266                 | 1 Affy CEL             | HG17              | in situ oligonucleotide |
| GSE19612 | 63 GPL3718,GPL3720,GPL9128 | 3 Affy CEL/Copy Number | HG17              | in situ oligonucleotide |
| GSE19647 | 159 GPL3718,GPL2005        | 2 Affy CEL             |                   | in situ oligonucleotide |
| GSE19714 | 5 GPL4091                  | 1 Log10                | HG17              | in situ oligonucleotide |
| GSE19730 | 70 GPL9852                 | 1 Log2                 | HG18              | spotted oligonucleotide |
| GSE19852 | 4 GPL4091                  | 1 Log10                | HG17              | in situ oligonucleotide |
| GSE1991  | 54 GPL1715                 | 1 Log2                 | Stanford IMAGE ID | spotted DNA/cDNA        |
| GSE19915 | 103 GPL4723                | 1 Log2                 | HG17              | BAC/P1                  |
| GSE19920 | 8 GPL3718,GPL3720          | 2 Affy CEL             | HG17              | in situ oligonucleotide |
| GSE19986 | 1 GPL6984                  | 1 LogR                 | HG18              | oligonucleotide beads   |
| GSE19996 | 48 GPL3718,GPL3720         | 2 Affy CEL             |                   | in situ oligonucleotide |
| GSE20154 | 56 GPL10001                | 1 Log2                 |                   | spotted oligonucleotide |
| GSE20239 | 3 GPL4091                  | 1 Log10                | HG17              | in situ oligonucleotide |
| GSE20353 | 86 GPL3718                 | 1 Affy CEL             | HG17              | oligonucleotide         |
| GSE20376 | 28 GPL2004,GPL2005         | 2 Affy CEL             |                   | in situ oligonucleotide |
| GSE20393 | 373 GPL9128                | 1 Signal Intensity     | HG17              | in situ oligonucleotide |
| GSE20394 | 167 GPL9128                | 1 Log2                 | HG17              | in situ oligonucleotide |
| GSE20474 | 8 GPL10093                 | 1 Log2                 |                   | spotted DNA/cDNA        |
| GSE20481 | 762 GPL2004,GPL2005        | 2 Affy CEL             |                   | in situ oligonucleotide |
| GSE20483 | 97 GPL9077                 | 1 Log2                 | HG17              | BAC/P1                  |
| GSE20496 | 98 GPL4560                 | 1 Log2                 |                   | BAC/P1                  |
| GSE20565 | 32 GPL2005,GPL6801         | 2 Affy CEL             | HG17/HG18         | in situ oligonucleotide |
| GSE20574 | 1 GPL9128                  | 1 Signal Intensity     | HG17              | in situ oligonucleotide |

GEO

|          |                             |            |                   |                         |
|----------|-----------------------------|------------|-------------------|-------------------------|
| GSE20584 | 2 GPL6801                   | 1 Affy CEL |                   | in situ oligonucleotide |
| GSE20634 | 29 GPL10118                 | 1 Log      | HG18              | in situ oligonucleotide |
| GSE20709 | 25 GPL6801                  | 1 Affy CEL |                   | in situ oligonucleotide |
| GSE20939 | 76 GPL3718,GPL3720          | 2 Affy CEL | HG17              | in situ oligonucleotide |
| GSE21025 | 19 GPL10150                 | 1 Log2     | HG18              | in situ oligonucleotide |
| GSE21035 | 231 GPL4091                 | 1 Log10    | HG17              | in situ oligonucleotide |
| GSE21057 | 92 GPL3718,GPL3720          | 2 Affy CEL |                   | in situ oligonucleotide |
| GSE21107 | 187 GPL6801                 | 1 Affy CEL |                   | in situ oligonucleotide |
| GSE21123 | 415 GPL3720                 | 1 Affy CEL |                   | in situ oligonucleotide |
| GSE21168 | 4 GPL8882                   | 1 LogR     |                   | oligonucleotide beads   |
| GSE21228 | 118 GPL6801                 | 1 Affy CEL | HG18              | in situ oligonucleotide |
| GSE21259 | 200 GPL4723,GPL7247,GPL9077 | 3 Log2     | HG17/HG17/HG17    | BAC/P1                  |
| GSE21347 | 18 GPL3718,GPL3720          | 2 Affy CEL |                   | in situ oligonucleotide |
| GSE21349 | 111 GPL3718,GPL3720         | 2 Affy CEL |                   | in situ oligonucleotide |
| GSE2139  | 94 GPL1432                  | 1 Log      | HG16              | BAC/P1                  |
| GSE21420 | 38 GPL4091                  | 1 Log2     | HG17              | in situ oligonucleotide |
| GSE21468 | 74 GPL4093,GPL10123         | 2 Log2     | HG17/HG18         | in situ oligonucleotide |
| GSE21530 | 8 GPL4091                   | 1 Log10    | HG17              | in situ oligonucleotide |
| GSE21540 | 7 GPL2616                   | 1 Log2     | HG15              | BAC/P1                  |
| GSE21554 | 21 GPL10383                 | 1 Log10    | HG18              | in situ oligonucleotide |
| GSE21597 | 99 GPL3718,GPL3720          | 2 Affy CEL |                   | in situ oligonucleotide |
| GSE21780 | 30 GPL6801                  | 1 Affy CEL |                   | in situ oligonucleotide |
| GSE21948 | 8 GPL10452                  | 1 Log2     | HG18              | spotted oligonucleotide |
| GSE21986 | 36 GPL9075                  | 1 Log2     | HG17              | in situ oligonucleotide |
| GSE21990 | 148 GPL6801                 | 1 Affy CEL |                   | in situ oligonucleotide |
| GSE22016 | 10 GPL10461                 | 1 Log2     | HG18              | in situ oligonucleotide |
| GSE22082 | 51 GPL3720                  | 1 Affy CEL |                   | in situ oligonucleotide |
| GSE22133 | 359 GPL4723,GPL7247         | 2 Log2     | HG17/HG17         | BAC/P1                  |
| GSE22185 | 25 GPL4093                  | 1 Log10    | HG17              | in situ oligonucleotide |
| GSE22208 | 48 GPL6801                  | 1 Affy CEL |                   | in situ oligonucleotide |
| GSE22221 | 15 GPL1831                  | 1 Log2     | Stanford IMAGE ID | spotted DNA/cDNA        |
| GSE22237 | 14 GPL9128                  | 1 Log10    | HG17              | in situ oligonucleotide |
| GSE22279 | 10 GPL9708                  | 1 Log      | HG18              | in situ oligonucleotide |
| GSE22305 | 22 GPL6801                  | 1 Affy CEL |                   | in situ oligonucleotide |

## GEO

|          |                            |                      |                |                                                 |
|----------|----------------------------|----------------------|----------------|-------------------------------------------------|
| GSE22401 | 26 GPL4560                 | 1 Log2               |                | BAC/P1                                          |
| GSE22461 | 3 GPL6801                  | 1 Affy CEL           | HG18           | in situ oligonucleotide                         |
| GSE22481 | 89 GPL4560                 | 1 Log2               |                | BAC/P1                                          |
| GSE22524 | 26 GPL4723                 | 1 Log2               | HG17           | BAC/P1                                          |
| GSE22547 | 1 GPL4091                  | 1 Log10              | HG17           | in situ oligonucleotide                         |
| GSE22577 | 4 GPL6804                  | 1 Affy CEL           |                | in situ oligonucleotide                         |
| GSE2258  | 54 GPL1855                 | 1 Affy               | HG15           | in situ oligonucleotide                         |
| GSE22615 | 15 GPL6801                 | 1 Affy CEL           | HG18           | in situ oligonucleotide                         |
| GSE22635 | 20 GPL5477                 | 1 Log10              | HG17           | in situ oligonucleotide                         |
| GSE22694 | 132 GPL4544                | 1 Log10              | HG17           | in situ oligonucleotide                         |
| GSE22785 | 14 GPL9128                 | 1 Log2               | HG17           | in situ oligonucleotide                         |
| GSE22839 | 22 GPL3720                 | 1 Affy CEL           |                | in situ oligonucleotide                         |
| GSE22905 | 3 GPL4091                  | 1 Log2               | HG17           | in situ oligonucleotide                         |
| GSE22916 | 100 GPL7313                | 1 Log2               | HG18           | in situ oligonucleotide                         |
| GSE22928 | 28 GPL6801,GPL6984,GPL9128 | 3 Affy CEL/Log2/LogR | HG18/HG18/HG17 | in situ oligonucleotide                         |
| GSE23005 | 31 GPL4091                 | 1 Log10              | HG17           | in situ oligonucleotide                         |
| GSE23065 | 2 GPL10123                 | 1 Log10              | HG18           | in situ oligonucleotide                         |
| GSE23300 | 91 GPL6801                 | 1 Affy CEL           |                | in situ oligonucleotide                         |
| GSE23452 | 226 GPL6801                | 1 Affy CEL           |                | in situ oligonucleotide                         |
| GSE23633 | 4 GPL4091                  | 1 Log10              | HG17           | in situ oligonucleotide                         |
| GSE23720 | 173 GPL9128                | 1 Log10              | HG17           | in situ oligonucleotide                         |
| GSE23785 | 9 GPL8887                  | 1 LogR               |                | oligonucleotide beads                           |
| GSE23823 | 13 GPL4091                 | 1 Log2               | HG17           | in situ oligonucleotide                         |
| GSE23831 | 60 GPL4093,GPL10722        | 2 Log2               | HG17           | in situ oligonucleotide                         |
| GSE23869 | 21 GPL6782                 | 1 Log2               | HG17           | BAC/P1                                          |
| GSE23891 | 25 GPL2879,GPL5477         | 2 Signal Intensity   | HG17/HG17      | in situ oligonucleotide/in situ oligonucleotide |
| GSE23946 | 39 GPL7823                 | 1 Log2               | HG17           | in situ oligonucleotide                         |
| GSE23949 | 4 GPL8736                  | 1 Log10              | HG18           | in situ oligonucleotide                         |
| GSE24144 | 6 GPL6801                  | 1 Affy               |                | in situ oligonucleotide                         |
| GSE24216 | 4 GPL4091                  | 1 Log10              | HG17           | in situ oligonucleotide                         |
| GSE24282 | 6 GPL4091                  | 1 Log10              | HG17           | in situ oligonucleotide                         |
| GSE24412 | 8 GPL3718,GPL3720          | 2 Affy CEL           |                | in situ oligonucleotide                         |
| GSE24446 | 11 GPL8736                 | 1 Log10              | HG18           | in situ oligonucleotide                         |
| GSE24452 | 14 GPL5477                 | 1 Log10              | HG17           | in situ oligonucleotide                         |

## GEO

|          |                                      |            |                     |                                                 |
|----------|--------------------------------------|------------|---------------------|-------------------------------------------------|
| GSE24602 | 107 GPL4091,GPL4093,GPL7823,GPL1012: | 4 Log10    | HG17/HG17/HG17/HG18 | in situ oligonucleotide                         |
| GSE24715 | 64 GPL3720,GPL2005                   | 2 Affy CEL |                     | in situ oligonucleotide                         |
| GSE24881 | 218 GPL3718                          | 1 Affy CEL |                     | in situ oligonucleotide                         |
| GSE24890 | 4 GPL6988                            | 1 LogR     | HG18                | oligonucleotide beads                           |
| GSE25016 | 291 GPL6801                          | 1 Affy CEL |                     | in situ oligonucleotide                         |
| GSE2520  | 128 GPL2014,GPL2015                  | 2 Affy CEL |                     | in situ oligonucleotide                         |
| GSE25298 | 25 GPL8841                           | 1 Log10    | HG17                | in situ oligonucleotide                         |
| GSE25399 | 90 GPL2004,GPL2005                   | 2 Affy CEL |                     | in situ oligonucleotide                         |
| GSE25411 | 1 GPL10123                           | 1 Log10    | HG18                | in situ oligonucleotide                         |
| GSE25528 | 20 GPL11237                          | 1 Log2     | HG19                | BAC/P1                                          |
| GSE25989 | 2 GPL6801                            | 1 Affy CEL |                     | in situ oligonucleotide                         |
| GSE26053 | 3 GPL6801                            | 1 Affy CEL | HG18                | in situ oligonucleotide                         |
| GSE26075 | 104 GPL3718,GPL3720,GPL2004,GPL2005  | 4 Affy CEL |                     | in situ oligonucleotide                         |
| GSE26301 | 2 GPL6801                            | 1 Affy CEL |                     | in situ oligonucleotide                         |
| GSE2631  | 126 GPL2024                          | 1 Log2     |                     | BAC/P1                                          |
| GSE26447 | 11 GPL9075                           | 1 Log10    | HG17                | in situ oligonucleotide                         |
| GSE26534 | 4 GPL9041                            | 1 Log2     | HG18                | in situ oligonucleotide                         |
| GSE2681  | 16 GPL2030                           | 1 Log2     |                     | BAC/P1                                          |
| GSE26849 | 254 GPL9128                          | 1 Log2     | HG17                | in situ oligonucleotide                         |
| GSE27193 | 9 GPL8887,GPL8888                    | 2 LogR     |                     | oligonucleotide beads                           |
| GSE27289 | 8 GPL13135                           | 1 LogR     |                     | oligonucleotide beads                           |
| GSE27331 | 46 GPL13176                          | 1 Log2     |                     | BAC/P1                                          |
| GSE27332 | 40 GPL13177                          | 1 Log2     | HG18                | BAC/P1                                          |
| GSE27392 | 26 GPL13190                          | 1 Log2     | HG18                | in situ oligonucleotide                         |
| GSE27636 | 17 GPL13244                          | 1 Log2     | HG17                | spotted DNA/cDNA                                |
| GSE27673 | 37 GPL9128                           | 1 Log2     | HG17                | in situ oligonucleotide                         |
| GSE28132 | 11 GPL6801                           | 1 Affy CEL | HG18                | in situ oligonucleotide                         |
| GSE28329 | 32 GPL2873,GPL4091                   | 2 Log10    | HG17/HG17           | in situ oligonucleotide/in situ oligonucleotide |
| GSE2922  | 28 GPL2043,GPL2616                   | 2 Log2     | HG17/HG15           | BAC/P1                                          |
| GSE2959  | 28 GPL1266,GPL2641                   | 2 Affy     | HG17                | in situ oligonucleotide                         |
| GSE3106  | 7 GPL2043,GPL2735                    | 2 Log2     | HG17                | BAC/P1                                          |
| GSE3281  | 59 GPL2830                           | 1 Log2     | Stanford IMAGE ID   | spotted DNA/cDNA                                |
| GSE3435  | 68 GPL2920                           | 1 Log      |                     | BAC/P1                                          |
| GSE3642  | 29 GPL3091                           | 1 Log2     | HG17                | BAC/P1                                          |

## GEO

|         |                                      |                             |                   |                                                         |
|---------|--------------------------------------|-----------------------------|-------------------|---------------------------------------------------------|
| GSE3743 | 78 GPL1266                           | 1 Affy CEL                  | HG17              | In situ oligonucleotide                                 |
| GSE3898 | 84 GPL1506                           | 1 Log2                      |                   | spotted DNA/cDNA                                        |
| GSE3930 | 17 GPL1282,GPL2790,GPL3254,GPL3291   | 4 Log2                      | Stanford IMAGE ID | spotted DNA/cDNA                                        |
| GSE4017 | 8 GPL3355                            | 1 Log2                      | Stanford IMAGE ID | spotted DNA/cDNA                                        |
| GSE4078 | 11 GPL3372,GPL3383                   | 2 Log2                      | Stanford IMAGE ID | spotted DNA/cDNA                                        |
| GSE4079 | 7 GPL3381,GPL3382,GPL3383            | 3 Log2                      | Stanford IMAGE ID | spotted DNA/cDNA                                        |
| GSE4173 | 17 GPL1448                           | 1 Log2                      | Stanford IMAGE ID | spotted DNA/cDNA                                        |
| GSE4176 | 27 GPL1266                           | 1 Affy                      | HG17              | In situ oligonucleotide                                 |
| GSE4244 | 9 GPL3455                            | 1 Log2                      | HG17              | BAC/P1                                                  |
| GSE4297 | 4 GPL3472,GPL3481                    | 2 Log2                      | HG17              | In situ oligonucleotide                                 |
| GSE4405 | 15 GPL3332,GPL3522,GPL3523,GPL3524,  | 5 Log2                      | Stanford IMAGE ID | spotted DNA/cDNA                                        |
| GSE4591 | 25 GPL2616                           | 1 Log2                      | HG15              | BAC/P1                                                  |
| GSE4659 | 32 GPL2873                           | 1 Log10                     | HG17              | In situ oligonucleotide                                 |
| GSE4747 | 16 GPL2024                           | 1 Log2                      |                   | BAC/P1                                                  |
| GSE4838 | 7 GPL3749                            | 1 Log2                      | HG17              | BAC/P1                                                  |
| GSE4860 | 8 GPL3778,GPL3780                    | 2 Log2                      |                   | BAC/P1                                                  |
| GSE4886 | 4 GPL3514                            | 1 Log2                      | HG17              | In situ oligonucleotide                                 |
| GSE49   | 5 GPL179                             | 1 Log2                      | Stanford IMAGE ID | spotted DNA/cDNA                                        |
| GSE5049 | 8 GPL2616                            | 1 Log2                      | HG15              | BAC/P1                                                  |
| GSE5051 | 167 GPL28,GPL2819,GPL2826,GPL2834,Gf | 8 Log2                      | HG17/HG16         | spotted oligonucleotide/spotted DNA/cDNA                |
| GSE5082 | 5 GPL1266                            | 1 Affy                      | HG17              | In situ oligonucleotide                                 |
| GSE5138 | 42 GPL3443                           | 1 Log2                      | HG16              | BAC/P1                                                  |
| GSE5316 | 48 GPL3789,GPL3868,GPL3869,GPL3993   | 4 Log2                      | HG17              | BAC/P1                                                  |
| GSE5336 | 109 GPL3887,GPL3888,GPL3889,GPL3892, | 7 Signal Intensity          |                   | spotted DNA/cDNA                                        |
| GSE5347 | 63 GPL1266,GPL2641,GPL3896,GPL4012   | 4 Affy CEL/Signal Intensity | HG17              | In situ oligonucleotide/BAC/P1                          |
| GSE5359 | 2 GPL3960                            | 1 Signal Intensity          | HG17              | BAC/P1                                                  |
| GSE5511 | 1099 GPL2004,GPL2005,GPL3720         | 3 Affy                      | HG17              | In situ oligonucleotide                                 |
| GSE5784 | 236 GPL4242                          | 1 Log2                      |                   | spotted DNA/cDNA                                        |
| GSE5927 | 41 GPL2005                           | 1 Affy                      |                   | In situ oligonucleotide                                 |
| GSE6040 | 18 GPL4453                           | 1 Log2                      | HG16              | spotted DNA/cDNA                                        |
| GSE6042 | 36 GPL2843                           | 1 Log2                      |                   | BAC/P1                                                  |
| GSE6109 | 356 GPL2004,GPL2005                  | Affy                        | HG17              | oligonucleotide/oligonucleotide/in situ oligonucleotide |
| GSE6123 | 10 GPL3898,GPL4482,GPL4483           | 3 Log2                      | Stanford IMAGE ID | spotted DNA/cDNA                                        |
| GSE6138 | 8 GPL3898                            | 1 Log2                      | Stanford IMAGE ID | spotted DNA/cDNA                                        |

## GEO

|         |                            |                    |                   |                                                         |
|---------|----------------------------|--------------------|-------------------|---------------------------------------------------------|
| GSE6145 | 16 GPL3898,GPL4505         | 2 Log2             | Stanford IMAGE ID | spotted DNA/cDNA                                        |
| GSE6415 | 2 GPL4544                  | 1 Log10            | HG17              | in situ oligonucleotide                                 |
| GSE6448 | 185 GPL3632                | 1 Log2             |                   | spotted DNA/cDNA                                        |
| GSE6469 | 64 GPL4639,GPL4640         | 2 Log2             | Stanford IMAGE ID | spotted DNA/cDNA                                        |
| GSE6473 | 15 GPL3441                 | 2 Log2             | HG16              | BAC/P1                                                  |
| GSE6567 | 24 GPL4615                 | 1 Log2             |                   | BAC/P1                                                  |
| GSE6713 | 23 GPL3892,GPL3894         | 2 Log2             |                   | BAC/P1                                                  |
| GSE6746 | 11 GPL4723                 | 1 Log2             | HG17              | BAC/P1                                                  |
| GSE6779 | 47 GPL4723                 | 1 Log2             | HG17              | BAC/P1                                                  |
| GSE7068 | 23 GPL2004,GPL2005         | 2 Affy CEL         | HG17              | oligonucleotide                                         |
| GSE7077 | 4 GPL2879                  | 1 Log              | HG17              | in situ oligonucleotide                                 |
| GSE7122 | 39 GPL4560                 | 1 Log2             |                   | BAC/P1                                                  |
| GSE7130 | 56 GPL2004,GPL2005         | 2 Affy CEL         | HG17              | oligonucleotide                                         |
| GSE7180 | 14 GPL4896                 | 1 Log2             |                   | BAC/P1                                                  |
| GSE7210 | 54 GPL1266,GPL2641         | 2 Affy CEL         | HG17              | in situ oligonucleotide                                 |
| GSE7230 | 82 GPL4894                 | 1 Signal Intensity |                   | BAC/P1                                                  |
| GSE7239 | 54 GPL4939                 | 1 Log2             |                   | BAC/P1                                                  |
| GSE7255 | 45 GPL2004,GPL2005,GPL3718 | 3 Affy CEL         | HG17              | oligonucleotide/oligonucleotide/in situ oligonucleotide |
| GSE7274 | 55 GPL4998,GPL4999         | 2 Log2             |                   | spotted DNA/cDNA                                        |
| GSE7344 | 16 GPL2873                 | 1 Log10            | HG17              | in situ oligonucleotide                                 |
| GSE7364 | 8 GPL570                   | 1 Signal Intensity |                   | in situ oligonucleotide                                 |
| GSE7376 | 11 GPL5046                 | 1 Log2             | HG16              | spotted oligonucleotide                                 |
| GSE7383 | 21 GPL2043,GPL2735         | 2 Log2             | HG17              | BAC/P1                                                  |
| GSE7408 | 27 GPL5015                 | 1 Log2             |                   | BAC/P1                                                  |
| GSE7425 | 61 GPL2641                 | 1 Affy CEL         | HG17              | in situ oligonucleotide                                 |
| GSE7426 | 12 GPL5055                 | 1 Log2             | HG17              | spotted DNA/cDNA                                        |
| GSE7427 | 96 GPL5056                 | 1 Log2             | HG17              | spotted DNA/cDNA                                        |
| GSE7482 | 25 GPL2879                 | 1 Log10            | HG17              | in situ oligonucleotide                                 |
| GSE7490 | 90 GPL1266                 | 1 Affy CEL         | HG17              | in situ oligonucleotide                                 |
| GSE7545 | 102 GPL3718,GPL3720        | 2 Affy CEL         | HG17              | in situ oligonucleotide                                 |
| GSE7599 | 30 GPL2879                 | 1 Log2             | HG17              | in situ oligonucleotide                                 |
| GSE7602 | 38 GPL2879                 | 1 Log2             | HG17              | in situ oligonucleotide                                 |
| GSE7603 | 26 GPL2879,GPL4091         | 2 Log2             | HG17              | in situ oligonucleotide                                 |
| GSE7604 | 81 GPL887                  | 1 Log2             |                   | in situ oligonucleotide                                 |

## GEO

|         |                                      |                    |  |                   |  |                                                           |
|---------|--------------------------------------|--------------------|--|-------------------|--|-----------------------------------------------------------|
| GSE7606 | 123 GPL887                           | 1 Log2             |  |                   |  | in situ oligonucleotide                                   |
| GSE7692 | 624 GPL4894                          | 1 Log2             |  |                   |  | BAC/P1                                                    |
| GSE7822 | 151 GPL2004,GPL2005,GPL2879,GPL3718, | 8 Affy CEL/Log2    |  | HG17/HG18         |  | in situ oligonucleotide/spotted oligonucleotide           |
| GSE7878 | 32 GPL2827                           | 1 Log2             |  | HG17              |  | spotted oligonucleotide                                   |
| GSE7882 | 111 GPL5326                          | 1 Log2             |  | HG17              |  | spotted oligonucleotide                                   |
| GSE7946 | 97 GPL1266,GPL2641                   | 2 Affy CEL         |  | HG17              |  | in situ oligonucleotide                                   |
| GSE7949 | 21 GPL5338                           | 1 Log2             |  | HG18              |  | BAC/P1                                                    |
| GSE8026 | 64 GPL2013                           | 1 Log2             |  | Stanford IMAGE ID |  | spotted DNA/cDNA                                          |
| GSE8046 | 25 GPL2005                           | 1 Affy CEL         |  | HG17              |  | in situ oligonucleotide                                   |
| GSE8067 | 149 GPL2843,GPL3441,GPL3442,GPL3443  | 4 Log2             |  | HG16              |  | BAC/P1                                                    |
| GSE8123 | 45 GPL2641                           | 1 Affy CEL         |  | HG17              |  | in situ oligonucleotide                                   |
| GSE8271 | 14 GPL2004,GPL2005                   | 2 Affy CEL         |  | HG17              |  | oligonucleotide                                           |
| GSE8333 | 44 GPL1266,GPL2641                   | 2 Affy CEL         |  | HG17              |  | in situ oligonucleotide                                   |
| GSE8351 | 67 GPL5452                           | 1 Log2             |  |                   |  | BAC/P1                                                    |
| GSE8398 | 25 GPL2879                           | 1 Log2             |  | HG17              |  | in situ oligonucleotide                                   |
| GSE8508 | 1 GPL3811                            | 1 Affy CEL         |  | HG17              |  | in situ oligonucleotide                                   |
| GSE8567 | 17 GPL2005                           | 1 Affy CEL         |  | HG17              |  | in situ oligonucleotide                                   |
| GSE8591 | 20 GPL5672                           | 1 Log2             |  | HG18              |  | BAC/P1                                                    |
| GSE8598 | 22 GPL5672                           | 1 Log2             |  | HG18              |  | BAC/P1                                                    |
| GSE8605 | 20 GPL2641,GPL4012                   | 2 Affy CEL/Log2    |  | HG17              |  | spotted DNA/cDNA                                          |
| GSE8614 | 74 GPL5679                           | 1 Log2             |  |                   |  | BAC/P1                                                    |
| GSE8628 | 24 GPL5477,GPL5571                   | 2 Signal Intensity |  | HG17              |  | in situ oligonucleotide                                   |
| GSE8634 | 80 GPL5685                           | 1 Log2             |  |                   |  | BAC/P1                                                    |
| GSE8649 | 8 GPL3718,GPL3720                    | 2 Affy CEL         |  | HG17              |  | in situ oligonucleotide                                   |
| GSE8721 | 467 GPL2641                          | 1 Affy CEL         |  | HG17              |  | in situ oligonucleotide                                   |
| GSE8736 | 10 GPL5685                           | 1 Log2             |  |                   |  | BAC/P1                                                    |
| GSE8737 | 66 GPL5713                           | 1 Log2             |  |                   |  | BAC/P1                                                    |
| GSE8738 | 73 GPL5713                           | 1 Log2             |  |                   |  | BAC/P1                                                    |
| GSE8757 | 220 GPL5737                          | 1 Log2             |  | HG18              |  | spotted oligonucleotide                                   |
| GSE8777 | 16 GPL3895                           | 1 Log2             |  | Stanford IMAGE ID |  | spotted DNA/cDNA                                          |
| GSE8798 | 28 GPL2005,GPL5749,GPL5750           | 3 Affy CEL/Log2    |  |                   |  | in situ oligonucleotide/spotted DNA/cDNA/spotted DNA/cDNA |
| GSE8801 | 71 GPL4999                           | 1 Log2             |  |                   |  | spotted DNA/cDNA                                          |
| GSE8804 | 13 GPL2873,GPL2879                   | 2 Log2             |  | HG17/HG17         |  | in situ oligonucleotide/in situ oligonucleotide           |
| GSE8855 | 2 GPL5790                            | 1 Log2             |  | HG17              |  | in situ oligonucleotide                                   |

## GEO

|         |                                      |            |                   |                                         |
|---------|--------------------------------------|------------|-------------------|-----------------------------------------|
| GSE8918 | 87 GPL2879                           | 1 Log2     | HG17              | in situ oligonucleotide                 |
| GSE8933 | 10 GPL4894                           | 1 Log2     |                   | BAC/P1                                  |
| GSE9003 | 76 GPL5711                           | 1 LogR     | HG17              | spotted oligonucleotide                 |
| GSE9021 | 37 GPL4560                           | 1 Log2     |                   | BAC/P1                                  |
| GSE9023 | 25 GPL5840,GPL5841                   | 2 Log2     | HG17              | BAC/P1                                  |
| GSE9109 | 1112 GPL2004,GPL2005,GPL3718,GPL3720 | 4 Affy     | HG17              | oligonucleotide/in situ oligonucleotide |
| GSE9110 | 112 GPL3718,GPL3720                  | 2 Affy     | HG17              | in situ oligonucleotide                 |
| GSE9111 | 200 GPL2004,GPL2005,GPL3718,GPL3720  | 4 Affy     | HG17              | oligonucleotide/in situ oligonucleotide |
| GSE9112 | 72 GPL3718,GPL3720                   | 2 Affy     | HG17              | in situ oligonucleotide                 |
| GSE9114 | 47 GPL4560                           | 1 Log2     |                   | BAC/P1                                  |
| GSE9154 | 42 GPL3720                           | 1 Affy CEL | HG17              | in situ oligonucleotide                 |
| GSE9177 | 11 GPL4091                           | 1 Log2     | HG17              | in situ oligonucleotide                 |
| GSE9193 | 94 GPL2043,GPL2616                   | 2 Log2     | HG17/HG15         | BAC/P1                                  |
| GSE9205 | 5 GPL5620                            | 1 Log2     | Stanford IMAGE ID | spotted DNA/cDNA                        |
| GSE9469 | 20 GPL2641                           | 1 Affy CEL | HG17              | in situ oligonucleotide                 |
| GSE9585 | 68 GPL2004,GPL2005,GPL3718,GPL3720   | 4 Affy CEL | HG17              | oligonucleotide/in situ oligonucleotide |
| GSE9611 | 165 GPL2641,GPL3718,GPL3720          | 3 Affy CEL | HG17              | in situ oligonucleotide                 |
| GSE9635 | 374 GPL2004,GPL2005                  | 2 Affy CEL | HG17              | oligonucleotide                         |
| GSE9654 | 10 GPL2879                           | 1 Log2     | HG17              | in situ oligonucleotide                 |
| GSE9672 | 52 GPL6181                           | 1 Log2     | Ensembl Ver49     | BAC/P1                                  |
| GSE9845 | 197 GPL3720                          | 1 Affy CEL | HG17              | in situ oligonucleotide                 |
| GSE9928 | 12 GPL5000                           | 1 Log      | HG17              | BAC/P1                                  |

ArrayExpress

| AE accession | Array No | Platform ID                         | Platform No | Data Type        | Genome Version | Array Type              |
|--------------|----------|-------------------------------------|-------------|------------------|----------------|-------------------------|
| E-MEXP-335   | 19       | A-MEXP-172                          | 1           | Signal Intensity |                | spotted DNA/cDNA        |
| E-MEXP-1852  | 24       | A-MEXP-1437,A-MEXP-1438,A-MEXP-1439 | 3           | Log2             | HG18           | in situ oligonucleotide |
| E-TABM-10    | 206      | A-MEXP-192                          | 1           | Log2             | HG17           | BAC/P1                  |
| E-TABM-65    | 60       | A-MEXP-285                          | 1           | Log2             |                | BAC/P1                  |
| E-TABM-246   | 29       | A-MEXP-285                          | 1           | Log2             |                | BAC/P1                  |
| E-TABM-267   | 17       | A-AGIL-20                           | 1           | Log2             | HG17           | in situ oligonucleotide |
| E-TABM-359   | 5        | A-MEXP-870,A-MEXP-885               | 2           | Log2             |                | BAC/P1                  |
| E-TABM-584   | 2        | A-MEXP-1544                         | 1           |                  |                | oligonucleotide beads   |
| E-TABM-712   | 67       | A-MEXP-1595,A-MEXP-1596             | 2           | Signal Intensity | HG18           | in situ oligonucleotide |
| E-TABM-857   | 53       | A-MEXP-1734                         | 1           | Log2             |                | BAC/P1                  |
| E-TABM-930   | 99       | A-MEXP-253,A-MEXP-341               | 2           | Log2             | Ensembl Ver33  | BAC/P1                  |

**Supplementary Table S2: Cancer entities grouped by ICD-O code**

| <b>Morphology</b>                                              | <b>ICD-O code</b> | <b>Number of samples</b> |
|----------------------------------------------------------------|-------------------|--------------------------|
| Infiltrating duct carcinoma, NOS                               | 8500/3            | 6459                     |
| Adenocarcinoma, NOS                                            | 8140/3            | 4826                     |
| Acute myeloid leukemia, NOS                                    | 9861/3            | 2147                     |
| Glioblastoma, NOS                                              | 9440/3            | 1989                     |
| Acute lymphoblastic leukemia, NOS                              | 9835/3            | 1614                     |
| Squamous cell carcinoma, NOS                                   | 8070/3            | 1359                     |
| Non-small cell carcinoma                                       | 8046/3            | 965                      |
| Neuroblastoma, NOS                                             | 9500/3            | 908                      |
| Medulloblastoma, NOS                                           | 9470/3            | 898                      |
| Carcinoma, NOS                                                 | 8010/3            | 873                      |
| Malignant melanoma, NOS                                        | 8720/3            | 844                      |
| Clear cell renal cell carcinoma                                | 8310/3            | 737                      |
| B-cell chronic lymphocytic leukemia/small lymphocytic lymphoma | 9823/3            | 708                      |
| Diffuse large B-cell lymphoma, NOS                             | 9680/3            | 638                      |
| Plasma cell myeloma                                            | 9732/3            | 559                      |
| follicular lymphoma, NOS                                       | 9690/3            | 558                      |
| Multiple myeloma                                               | 9731/3            | 558                      |
| Myelodysplastic syndrome, NOS                                  | 9989/3            | 551                      |
| Micropapillary serous carcinoma [C56.9]                        | 8460/3            | 513                      |
| Hepatocellular carcinoma, NOS                                  | 8170/3            | 488                      |
| Endometroid carcinoma, NOS                                     | 8380/3            | 433                      |
| Chronic myeloid leukemia, NOS                                  | 9863/3            | 330                      |
| Marginal zone lymphoma, NOS                                    | 9699/3            | 289                      |
| Renal cell carcinoma                                           | 8312/3            | 286                      |
| Mantle cell lymphoma                                           | 9673/3            | 278                      |
| Transitional cell carcinoma, NOS                               | 8120/3            | 241                      |
| Gastrointestinal stromal tumor, malignant                      | 8936/3            | 233                      |
| Splenic marginal zone lymphoma, NOS                            | 9689/3            | 204                      |
| Ductal carcinoma in situ, NOS                                  | 8500/2            | 179                      |
| Adenoma, NOS                                                   | 8140/0            | 179                      |
| Primitive neuroectodermal tumor, NOS                           | 9473/3            | 179                      |
| Chronic myeloproliferative disease, NOS                        | 9960/3            | 173                      |
| Adenocarcinoma, intestinal type                                | 8144/3            | 167                      |

|                                                     |        |     |
|-----------------------------------------------------|--------|-----|
| Oligodendroglioma, NOS                              | 9450/3 | 160 |
| Serous adenocarcinoma, NOS                          | 8441/3 | 155 |
| Pilocytic astrocytoma                               | 9421/1 | 154 |
| Glioma, NOS                                         | 9380/3 | 145 |
| Astrocytoma, NOS                                    | 9400/3 | 143 |
| Ependymoma, NOS                                     | 9391/3 | 137 |
| Medulloblastoma with extensive nodularity           | 9471/3 | 133 |
| Osteosarcoma, NOS                                   | 9180/3 | 108 |
| Peripheral T-cell lymphoma, NOS                     | 9705/3 | 108 |
| Small cell carcinoma, NOS                           | 8041/3 | 100 |
| Malignant lymphoma, B-cell NOS                      | 9591/3 | 99  |
| Precursor T-cell lymphoblastic leukemia             | 9837/3 | 99  |
| Leiomyosarcoma, NOS                                 | 8890/3 | 93  |
| Acute leukemia, NOS                                 | 9801/3 | 86  |
| Astrocytoma, anaplastic                             | 9401/3 | 80  |
| Large cell medulloblastoma                          | 9474/3 | 77  |
| Burkitt lymphoma, NOS                               | 9687/3 | 76  |
| Alveolar rhabdomyosarcoma                           | 8920/3 | 74  |
| Chondrosarcoma, NOS                                 | 9220/3 | 73  |
| Neurofibroma, NOS                                   | 9540/0 | 73  |
| Chronic myelomonocytic leukemia, NOS                | 9945/3 | 73  |
| Mucinous adenocarcinoma                             | 8480/3 | 70  |
| mycosis fungoides                                   | 9700/3 | 63  |
| Atypical chronic myeloid leukemia, BCR/ABL negative | 9876/3 | 63  |
| papillary renal cell carcinoma                      | 8260/3 | 63  |
| Invasive lobular carcinoma                          | 8520/3 | 62  |
| Mesothelioma, NOS                                   | 9050/3 | 60  |
| Acute promyelocytic leukemia [FAB type M3]          | 9866/3 | 56  |
| Oligodendroglioma, anaplastic                       | 9451/3 | 55  |
| Glioma, mixed                                       | 9382/3 | 55  |
| Ewing sarcoma                                       | 9260/3 | 52  |
| Liposarcoma, dedifferentiated                       | 8858/3 | 51  |
| Chordoma, NOS                                       | 9370/3 | 49  |
| Chronic idiopathic myelofibrosis                    | 9961/3 | 48  |
| Fibrosarcoma, NOS                                   | 8810/3 | 47  |
| Sezary syndrome                                     | 9701/3 | 46  |
| Squamous intraepithelial neoplasia, grade III       | 8077/2 | 46  |

|                                                           |        |    |
|-----------------------------------------------------------|--------|----|
| Embryonal rhabdomyosarcoma                                | 8910/3 | 46 |
| Polycythemia vera                                         | 9950/3 | 45 |
| Essential thrombocythemia                                 | 9962/3 | 45 |
| Infiltrating duct and lobular carcinoma                   | 8522/3 | 44 |
| Malignant peripheral nerve sheath tumor                   | 9540/3 | 44 |
| Myxoinflammatory fibroblastic sarcoma                     | 8811/3 | 43 |
| Waldenstrom macroglobulinemia                             | 9761/3 | 42 |
| Mediastinal large B-cell lymphoma                         | 9679/3 | 40 |
| Liposarcoma, NOS                                          | 8850/3 | 38 |
| Urothelial papilloma, NOS                                 | 8130/1 | 38 |
| Adrenal cortical carcinoma                                | 8370/3 | 36 |
| Mixed germ cell tumor                                     | 9085/3 | 36 |
| Undifferentiated sarcoma                                  | 8805/3 | 34 |
| Medullary carcinoma, NOS                                  | 8510/3 | 33 |
| Acute lymphoblastic leukemia, mature B-cell type          | 9826/3 | 31 |
| Enteropathy type T-cell lymphoma                          | 9717/3 | 31 |
| Teratoma, malignant, NOS                                  | 9080/3 | 30 |
| Lobular carcinoma in situ                                 | 8520/2 | 28 |
| Basal cell carcinoma, NOS                                 | 8090/3 | 28 |
| Merkel cell carcinoma                                     | 8247/3 | 26 |
| Acute monoblastic leukemia with differentiation [FAB M5b] | 9891/3 | 26 |
| Retinoblastoma, NOS                                       | 9510/3 | 24 |
| Liposarcoma, pleomorphic                                  | 8854/3 | 24 |
| Sarcoma, NOS                                              | 8800/3 | 22 |
| Superficial spreading melanoma                            | 8743/3 | 22 |
| Liposarcoma, myxoid                                       | 8852/3 | 21 |
| Epithelial tumor, benign                                  | 8010/0 | 21 |
| Carcinoma in situ, NOS                                    | 8010/2 | 20 |
| Ganglioglioma                                             | 9505/1 | 20 |
| Synovial sarcoma, monophasic                              | 9041/3 | 20 |
| Renal cell carcinoma, chromophobe                         | 8317/3 | 19 |
| Myoepithelioma                                            | 8982/0 | 19 |
| Adenosquamous carcinoma                                   | 8560/3 | 19 |
| Yolk sac tumor                                            | 9071/3 | 18 |
| Oncocytoma                                                | 8290/0 | 18 |
| Refractory anemia, NOS                                    | 9980/3 | 18 |
| Rhabdomyosarcoma, NOS                                     | 8900/3 | 17 |

|                                                                     |        |    |
|---------------------------------------------------------------------|--------|----|
| Pigmented dermatofibrosarcoma protuberans                           | 8833/3 | 17 |
| Seminoma, NOS                                                       | 9061/3 | 17 |
| Leukemia, NOS                                                       | 9800/3 | 16 |
| Intratubular germ cell neoplasia [C62.]                             | 9064/2 | 16 |
| Pineoblastoma                                                       | 9362/3 | 16 |
| Gastrointestinal stromal tumor, uncertain malignant potential       | 8936/1 | 15 |
| Epithelioid mesothelioma, malignant                                 | 9052/3 | 15 |
| Myoepithelial carcinoma                                             | 8562/3 | 14 |
| Teratocarcinoma                                                     | 9081/3 | 13 |
| Olfactory neuroblastoma                                             | 9522/3 | 13 |
| Pituitary carcinoma, NOS                                            | 8272/3 | 13 |
| Precursor T-cell lymphoblastic lymphoma                             | 9729/3 | 12 |
| Prolymphocytic leukemia, T-cell type                                | 9834/3 | 12 |
| Hodgkin lymphoma, NOS                                               | 9650/3 | 12 |
| Teratoma, benign                                                    | 9080/0 | 12 |
| Malignant lymphoma, NOS                                             | 9590/3 | 12 |
| Hepatoblastoma                                                      | 8970/3 | 12 |
| Angiosarcoma                                                        | 9120/3 | 11 |
| Refractory anemia with ringed sideroblasts [RARS]                   | 9982/3 | 11 |
| Acute myeloblastic leukemia with maturation [FAB M2]                | 9874/3 | 11 |
| Malignant lymphoma, lymphoplasmacytic                               | 9671/3 | 10 |
| Embryonal carcinoma, NOS                                            | 9070/3 | 9  |
| Chondroblastic osteosarcoma                                         | 9181/3 | 8  |
| Desmoplastic mesothelioma                                           | 9051/3 | 8  |
| Precursor B-cell lymphoblastic lymphoma                             | 9728/3 | 7  |
| Large cell carcinoma, NOS                                           | 8012/3 | 7  |
| Dendritic cell sarcoma, NOS                                         | 9757/3 | 7  |
| Ductal carcinoma, cribriform type [C50.]                            | 8201/3 | 7  |
| meningioma, NOS                                                     | 9530/0 | 7  |
| Nephroblastoma, NOS                                                 | 8960/3 | 7  |
| Acute megakaryoblastic leukemia [FAB M7]                            | 9910/3 | 7  |
| Intraductal papillary-mucinous adenoma [C25.]                       | 8453/0 | 7  |
| Carcinoma, diffuse type                                             | 8145/3 | 7  |
| Synovial sarcoma, NOS                                               | 9040/3 | 6  |
| Acute myeloblastic leukemia without maturation [FAB type M1]        | 9873/3 | 6  |
| Schwannoma, NOS                                                     | 9560/0 | 5  |
| Intraductal papillary-mucinous tumor with moderate dysplasia [C25.] | 8453/1 | 5  |

|                                                                 |        |   |
|-----------------------------------------------------------------|--------|---|
| Intraductal papillary-mucinous carcinoma, non-invasive [C25. _] | 8453/2 | 5 |
| Nodular melanoma                                                | 8721/3 | 4 |
| Refractory cytopenia with multilineage dysplasia                | 9985/3 | 4 |
| Intraductal papillary-mucinous carcinoma, invasive [C25. _]     | 8453/3 | 4 |
| Synovial sarcoma, biphasic                                      | 9043/3 | 4 |
| Basaloid squamous cell carcinoma                                | 8083/3 | 4 |
| Carcinoma, undifferentiated type, NOS                           | 8020/3 | 3 |
| Hepatocellular adenoma, NOS                                     | 8170/0 | 3 |
| Gliosarcoma                                                     | 9442/3 | 3 |
| Germ cell tumor, nonseminomatous                                | 9065/3 | 3 |
| Fibroblastic osteosarcoma                                       | 9182/3 | 3 |
| Precursor B-cell lymphoblastic leukemia                         | 9836/3 | 3 |
| Myelodysplastic syndrome with 5q- syndrome                      | 9986/3 | 3 |
| Refractory anemia with excess blasts [RAEB]                     | 9983/3 | 3 |
| Mesothelioma, biphasic, malignant                               | 9053/3 | 3 |
| Hypereosinophilic syndrome                                      | 9964/3 | 3 |
| Tubular adenocarcinoma                                          | 8211/3 | 3 |
| Epithelioma, malignant                                          | 8011/3 | 2 |
| Carcinosarcoma, NOS                                             | 8980/3 | 2 |
| Granular cell tumor                                             | 9582/0 | 2 |
| DCIS, comedo type [C50. _]                                      | 8501/2 | 2 |
| Hemangioma, NOS                                                 | 9120/0 | 2 |
| Metaplastic carcinoma, NOS                                      | 8575/3 | 2 |
| Inflammatory carcinoma                                          | 8530/3 | 2 |
| Carcinoma, anaplastic type, NOS                                 | 8021/3 | 2 |
| Acute myelomonocytic leukemia [FAB type M4]                     | 9867/3 | 2 |
| Atypical teratoid/rhabdoid tumor                                | 9508/3 | 2 |
| Meningioma, malignant                                           | 9530/3 | 2 |
| Sarcomatoid carcinoma                                           | 8033/3 | 2 |
| Pleomorphic xanthoastrocytoma                                   | 9424/3 | 2 |
| Papillary transitional cell carcinoma                           | 8130/3 | 2 |
| Acinar cell carcinoma                                           | 8550/3 | 2 |
| Endometrioid adenocarcinoma, secretory variant                  | 8382/3 | 2 |
| Germioma                                                        | 9064/3 | 1 |
| Choriocarcinoma                                                 | 9100/3 | 1 |
| Myeloid leukemia, NOS                                           | 9860/3 | 1 |
| Infiltrating lobular mixed with other types of carcinoma        | 8524/3 | 1 |

|                                                                |              |   |
|----------------------------------------------------------------|--------------|---|
| Adenocarcinoma in adenomatous polyp                            | 8210/3       | 1 |
| Osteosarcoma, telangiectatic                                   | 9183/3       | 1 |
| Refractory anemia with excess blasts in transformation [RAEBT] | 9984/3       | 1 |
| Dysgerminoma                                                   | 9060/3       | 1 |
| Phyllodes tumor, malignant                                     | 9020/3       | 1 |
| Desmoplastic fibroma                                           | 8823/0       | 1 |
| Fibrous histiocytoma, malignant                                | 8830/3       | 1 |
| Inflammatory myofibroblastic tumour                            | 8825/1       | 1 |
| Solid carcinoma, NOS                                           | 8230/3       | 1 |
| Apocrine adenocarcinoma                                        | 8401/3       | 1 |
| Infiltrating duct mixed with other types of carcinoma [C50.]   | 8523/3       | 1 |
| Paget disease and infiltrating duct carcinoma                  | 8541/3       | 1 |
| Bronchiolo-alveolar carcinoma, non-mucinous                    | 8252/3       | 1 |
| <b>Total</b>                                                   | <b>36078</b> |   |

**Supplementary Table S3: Platform type distribution in arrayMap**

| <b>Platform type</b>    | <b>Number of platform</b> |
|-------------------------|---------------------------|
| BAC/P1                  | 62                        |
| In situ oligonucleotide | 63                        |
| oligonucleotide beads   | 12                        |
| spotted DNA/cDNA        | 86                        |
| spotted oligonucleotide | 19                        |
| <b>Total</b>            | <b>242</b>                |

Supplementary Table S4: Probe remapping rate for platforms

| GPLID   | GenomeVersion | ArrayType | SANGER/DECIPHER | UCSC database | IMAGEID clone | Total |
|---------|---------------|-----------|-----------------|---------------|---------------|-------|
| GPL6181 | Ensembl Ver49 | BAC/P1    | 100%            |               |               | 100%  |
| GPL2616 | HG15          | BAC/P1    |                 | 99%           |               | 99%   |
| GPL1432 | HG16          | BAC/P1    | 100%            |               |               | 100%  |
| GPL2843 | HG16          | BAC/P1    | 97%             | 3%            |               | 100%  |
| GPL3441 | HG16          | BAC/P1    | 89%             | 11%           |               | 100%  |
| GPL7298 | HG16          | BAC/P1    | 98%             |               |               | 98%   |
| GPL8186 | HG16          | BAC/P1    | 86%             | 14%           |               | 100%  |
| GPL8187 | HG16          | BAC/P1    | 91%             | 9%            |               | 100%  |
| GPL2735 | HG17          | BAC/P1    |                 | 98%           |               | 98%   |
| GPL3091 | HG17          | BAC/P1    | 98%             | 2%            |               | 100%  |
| GPL3455 | HG17          | BAC/P1    | 97%             | 3%            |               | 100%  |
| GPL3749 | HG17          | BAC/P1    | 81%             | 19%           |               | 100%  |
| GPL3789 | HG17          | BAC/P1    | 63%             |               |               | 63%   |
| GPL3868 | HG17          | BAC/P1    | 97%             |               |               | 97%   |
| GPL3869 | HG17          | BAC/P1    | 97%             |               |               | 97%   |
| GPL3960 | HG17          | BAC/P1    | 81%             | 19%           |               | 100%  |
| GPL3993 | HG17          | BAC/P1    | 97%             |               |               | 97%   |
| GPL4723 | HG17          | BAC/P1    | 78%             | 20%           |               | 98%   |
| GPL5000 | HG17          | BAC/P1    | 78%             | 22%           |               | 100%  |
| GPL5114 | HG17          | BAC/P1    | 80%             | 20%           |               | 100%  |
| GPL5840 | HG17          | BAC/P1    | 79%             |               |               | 79%   |
| GPL5841 | HG17          | BAC/P1    | 92%             |               |               | 92%   |
| GPL6520 | HG17          | BAC/P1    | 98%             | 2%            |               | 100%  |
| GPL6521 | HG17          | BAC/P1    | 98%             | 2%            |               | 100%  |
| GPL6737 | HG17          | BAC/P1    | 89%             | 2%            |               | 91%   |
| GPL6782 | HG17          | BAC/P1    | 100%            |               |               | 100%  |
| GPL6783 | HG17          | BAC/P1    | 94%             | 6%            |               | 100%  |
| GPL7247 | HG17          | BAC/P1    | 79%             | 20%           |               | 99%   |
| GPL7394 | HG17          | BAC/P1    | 84%             | 15%           |               | 99%   |
| GPL8634 | HG17          | BAC/P1    | 91%             | 6%            |               | 97%   |
| GPL9077 | HG17          | BAC/P1    | 82%             | 18%           |               | 100%  |

|          |      |                         |      |     |    |      |
|----------|------|-------------------------|------|-----|----|------|
| GPL13177 | HG18 | BAC/P1                  | NA   | NA  | NA | NA   |
| GPL5338  | HG18 | BAC/P1                  | NA   | NA  | NA | NA   |
| GPL5672  | HG18 | BAC/P1                  | NA   | NA  | NA | NA   |
| GPL5772  | HG18 | BAC/P1                  | NA   | NA  | NA | NA   |
| GPL6853  | HG18 | BAC/P1                  | NA   | NA  | NA | NA   |
| GPL8690  | HG18 | BAC/P1                  | NA   | NA  | NA | NA   |
| GPL9715  | HG18 | BAC/P1                  | NA   | NA  | NA | NA   |
| GPL1003  |      | BAC/P1                  | 100% |     |    | 100% |
| GPL1005  |      | BAC/P1                  | 100% |     |    | 100% |
| GPL1048  |      | BAC/P1                  | 100% |     |    | 100% |
| GPL13176 |      | BAC/P1                  | NA   | NA  | NA | NA   |
| GPL2024  |      | BAC/P1                  | 99%  |     |    | 99%  |
| GPL2030  |      | BAC/P1                  | 91%  | 9%  |    | 100% |
| GPL2043  |      | BAC/P1                  |      | 98% |    | 98%  |
| GPL28    |      | BAC/P1                  | 70%  | 26% |    | 96%  |
| GPL2920  |      | BAC/P1                  | 99%  | 0%  |    | 99%  |
| GPL3778  |      | BAC/P1                  | 80%  | 19% |    | 99%  |
| GPL3780  |      | BAC/P1                  | 88%  | 10% |    | 98%  |
| GPL4560  |      | BAC/P1                  | 97%  |     |    | 97%  |
| GPL4615  |      | BAC/P1                  | 97%  |     |    | 97%  |
| GPL4894  |      | BAC/P1                  | 78%  | 22% |    | 100% |
| GPL4896  |      | BAC/P1                  | 99%  |     |    | 99%  |
| GPL4939  |      | BAC/P1                  | 97%  | 3%  |    | 100% |
| GPL5015  |      | BAC/P1                  | 95%  | 5%  |    | 100% |
| GPL5452  |      | BAC/P1                  | 100% |     |    | 100% |
| GPL5679  |      | BAC/P1                  | 91%  |     |    | 91%  |
| GPL5685  |      | BAC/P1                  | 100% |     |    | 100% |
| GPL5713  |      | BAC/P1                  | 100% |     |    | 100% |
| GPL6575  |      | BAC/P1                  | 100% |     |    | 100% |
| GPL7096  |      | BAC/P1                  | 97%  |     |    | 97%  |
| GPL8175  |      | BAC/P1                  | 100% |     |    | 100% |
| GPL1855  | HG15 | in situ oligonucleotide | NA   | NA  | NA | NA   |
| GPL9797  | HG16 | in situ oligonucleotide | 100% |     |    | 100% |
| GPL1266  | HG17 | in situ oligonucleotide | NA   | NA  | NA | NA   |

|          |      |                         |      |      |    |      |
|----------|------|-------------------------|------|------|----|------|
| GPL2004  | HG17 | in situ oligonucleotide | NA   | NA   | NA | NA   |
| GPL2005  | HG17 | in situ oligonucleotide | NA   | NA   | NA | NA   |
| GPL2641  | HG17 | in situ oligonucleotide | NA   | NA   | NA | NA   |
| GPL2873  | HG17 | in situ oligonucleotide | 100% |      |    | 100% |
| GPL2879  | HG17 | in situ oligonucleotide | 100% |      |    | 100% |
| GPL3472  | HG17 | in situ oligonucleotide |      | 100% |    | 100% |
| GPL3481  | HG17 | in situ oligonucleotide |      | 100% |    | 100% |
| GPL3514  | HG17 | in situ oligonucleotide |      | 100% |    | 100% |
| GPL3718  | HG17 | in situ oligonucleotide | NA   | NA   | NA | NA   |
| GPL3720  | HG17 | in situ oligonucleotide | NA   | NA   | NA | NA   |
| GPL3811  | HG17 | in situ oligonucleotide | NA   | NA   | NA | NA   |
| GPL4091  | HG17 | in situ oligonucleotide | 100% |      |    | 100% |
| GPL4093  | HG17 | in situ oligonucleotide | 100% |      |    | 100% |
| GPL4544  | HG17 | in situ oligonucleotide | 100% |      |    | 100% |
| GPL5477  | HG17 | in situ oligonucleotide | 100% |      |    | 100% |
| GPL5571  | HG17 | in situ oligonucleotide | 100% |      |    | 100% |
| GPL5790  | HG17 | in situ oligonucleotide |      | 100% |    | 100% |
| GPL6400  | HG17 | in situ oligonucleotide |      | 100% |    | 100% |
| GPL7203  | HG17 | in situ oligonucleotide | 100% |      |    | 100% |
| GPL7823  | HG17 | in situ oligonucleotide | 100% |      |    | 100% |
| GPL8581  | HG17 | in situ oligonucleotide |      | 100% |    | 100% |
| GPL8720  | HG17 | in situ oligonucleotide |      | 100% |    | 100% |
| GPL8841  | HG17 | in situ oligonucleotide | 100% |      |    | 100% |
| GPL9075  | HG17 | in situ oligonucleotide | 100% |      |    | 100% |
| GPL9128  | HG17 | in situ oligonucleotide | 100% |      |    | 100% |
| GPL9775  | HG17 | in situ oligonucleotide |      | 100% |    | 100% |
| GPL9776  | HG17 | in situ oligonucleotide |      | 100% |    | 100% |
| GPL9798  | HG17 | in situ oligonucleotide | 100% |      |    | 100% |
| GPL9816  | HG17 | in situ oligonucleotide |      | 100% |    | 100% |
| GPL10118 | HG18 | in situ oligonucleotide | NA   | NA   | NA | NA   |
| GPL10123 | HG18 | in situ oligonucleotide | NA   | NA   | NA | NA   |
| GPL10150 | HG18 | in situ oligonucleotide | NA   | NA   | NA | NA   |
| GPL10197 | HG18 | in situ oligonucleotide | NA   | NA   | NA | NA   |
| GPL10383 | HG18 | in situ oligonucleotide | NA   | NA   | NA | NA   |

|           |      |                         |      |     |    |    |      |
|-----------|------|-------------------------|------|-----|----|----|------|
| GPL 10461 | HG18 | in situ oligonucleotide | NA   | NA  | NA | NA | NA   |
| GPL 13190 | HG18 | in situ oligonucleotide | NA   | NA  | NA | NA | NA   |
| GPL6801   | HG18 | in situ oligonucleotide | NA   | NA  | NA | NA | NA   |
| GPL6804   | HG18 | in situ oligonucleotide | NA   | NA  | NA | NA | NA   |
| GPL7313   | HG18 | in situ oligonucleotide | NA   | NA  | NA | NA | NA   |
| GPL7314   | HG18 | in situ oligonucleotide | NA   | NA  | NA | NA | NA   |
| GPL8226   | HG18 | in situ oligonucleotide | NA   | NA  | NA | NA | NA   |
| GPL8233   | HG18 | in situ oligonucleotide | NA   | NA  | NA | NA | NA   |
| GPL8687   | HG18 | in situ oligonucleotide | NA   | NA  | NA | NA | NA   |
| GPL8736   | HG18 | in situ oligonucleotide | NA   | NA  | NA | NA | NA   |
| GPL8737   | HG18 | in situ oligonucleotide | NA   | NA  | NA | NA | NA   |
| GPL9041   | HG18 | in situ oligonucleotide | NA   | NA  | NA | NA | NA   |
| GPL9042   | HG18 | in situ oligonucleotide | NA   | NA  | NA | NA | NA   |
| GPL9708   | HG18 | in situ oligonucleotide | NA   | NA  | NA | NA | NA   |
| GPL9944   | HG18 | in situ oligonucleotide | NA   | NA  | NA | NA | NA   |
| GPL10722  |      | in situ oligonucleotide | 100% |     |    |    | 100% |
| GPL2014   |      | in situ oligonucleotide | NA   | NA  | NA | NA | NA   |
| GPL2015   |      | in situ oligonucleotide | NA   | NA  | NA | NA | NA   |
| GPL570    |      | in situ oligonucleotide | NA   | NA  | NA | NA | NA   |
| GPL8036   |      | in situ oligonucleotide | NA   | NA  | NA | NA | NA   |
| GPL8355   |      | in situ oligonucleotide | 100% |     |    |    | 100% |
| GPL8693   |      | in situ oligonucleotide | 100% |     |    |    | 100% |
| GPL887    |      | in situ oligonucleotide |      | 98% |    |    | 98%  |
| GPL9202   |      | in situ oligonucleotide | NA   | NA  | NA | NA | NA   |
| GPL6986   | HG18 | oligonucleotide         | NA   | NA  | NA | NA | NA   |
| GPL6979   | HG17 | oligonucleotide beads   | 100% |     |    |    | 100% |
| GPL6980   | HG18 | oligonucleotide beads   | NA   | NA  | NA | NA | NA   |
| GPL6981   | HG18 | oligonucleotide beads   | NA   | NA  | NA | NA | NA   |
| GPL6982   | HG18 | oligonucleotide beads   | NA   | NA  | NA | NA | NA   |
| GPL6984   | HG18 | oligonucleotide beads   | NA   | NA  | NA | NA | NA   |
| GPL6985   | HG18 | oligonucleotide beads   | NA   | NA  | NA | NA | NA   |
| GPL6988   | HG18 | oligonucleotide beads   | NA   | NA  | NA | NA | NA   |
| GPL 13135 |      | oligonucleotide beads   | NA   | NA  | NA | NA | NA   |
| GPL3896   |      | oligonucleotide beads   | NA   | NA  | NA | NA | NA   |

|          |                   |                       |      |     |     |      |
|----------|-------------------|-----------------------|------|-----|-----|------|
| GPL8882  |                   | oligonucleotide beads | NA   | NA  | NA  | NA   |
| GPL8887  |                   | oligonucleotide beads | NA   | NA  | NA  | NA   |
| GPL8888  |                   | oligonucleotide beads | NA   | NA  | NA  | NA   |
| GPL9336  | Ensembl 22.34d.1  | spotted DNA/cDNA      | 81%  |     |     | 81%  |
| GPL8774  | HG15              | spotted DNA/cDNA      |      | 99% |     | 99%  |
| GPL2842  | HG16              | spotted DNA/cDNA      | 89%  | 11% |     | 100% |
| GPL3442  | HG16              | spotted DNA/cDNA      | 89%  | 11% |     | 100% |
| GPL3443  | HG16              | spotted DNA/cDNA      | 86%  | 11% |     | 97%  |
| GPL13244 | HG17              | spotted DNA/cDNA      | 97%  |     |     | 97%  |
| GPL4012  | HG17              | spotted DNA/cDNA      | 96%  | 2%  |     | 98%  |
| GPL5055  | HG17              | spotted DNA/cDNA      | 100% |     |     | 100% |
| GPL5056  | HG17              | spotted DNA/cDNA      | 100% |     |     | 100% |
| GPL6088  | HG17              | spotted DNA/cDNA      | 79%  |     |     | 79%  |
| GPL6745  | HG17              | spotted DNA/cDNA      | NA   | NA  | NA  | NA   |
| GPL7199  | HG17              | spotted DNA/cDNA      | 100% |     |     | 100% |
| GPL6382  | HG18              | spotted DNA/cDNA      | NA   | NA  | NA  | NA   |
| GPL6478  | HG18              | spotted DNA/cDNA      | NA   | NA  | NA  | NA   |
| GPL6514  | HG18              | spotted DNA/cDNA      | NA   | NA  | NA  | NA   |
| GPL1282  | Stanford IMAGE ID | spotted DNA/cDNA      |      |     | 92% | 92%  |
| GPL1448  | Stanford IMAGE ID | spotted DNA/cDNA      |      |     | 90% | 90%  |
| GPL1715  | Stanford IMAGE ID | spotted DNA/cDNA      |      |     | 92% | 92%  |
| GPL179   | Stanford IMAGE ID | spotted DNA/cDNA      |      |     | 96% | 96%  |
| GPL1831  | Stanford IMAGE ID | spotted DNA/cDNA      |      |     | 92% | 92%  |
| GPL1998  | Stanford IMAGE ID | spotted DNA/cDNA      |      |     | 98% | 98%  |
| GPL2013  | Stanford IMAGE ID | spotted DNA/cDNA      |      |     | 98% | 98%  |
| GPL2790  | Stanford IMAGE ID | spotted DNA/cDNA      |      |     | 94% | 94%  |
| GPL2830  | Stanford IMAGE ID | spotted DNA/cDNA      |      |     | 97% | 97%  |
| GPL3254  | Stanford IMAGE ID | spotted DNA/cDNA      |      |     | 94% | 94%  |
| GPL3291  | Stanford IMAGE ID | spotted DNA/cDNA      |      |     | 92% | 92%  |
| GPL3332  | Stanford IMAGE ID | spotted DNA/cDNA      |      |     | 94% | 94%  |
| GPL3355  | Stanford IMAGE ID | spotted DNA/cDNA      |      |     | 92% | 92%  |
| GPL3372  | Stanford IMAGE ID | spotted DNA/cDNA      |      |     | 94% | 94%  |
| GPL3381  | Stanford IMAGE ID | spotted DNA/cDNA      |      |     | 92% | 92%  |
| GPL3382  | Stanford IMAGE ID | spotted DNA/cDNA      |      |     | 94% | 94%  |

|         |                   |                  |     |     |
|---------|-------------------|------------------|-----|-----|
| GPL3383 | Stanford IMAGE ID | spotted DNA/cDNA | 94% | 94% |
| GPL3522 | Stanford IMAGE ID | spotted DNA/cDNA | 92% | 92% |
| GPL3523 | Stanford IMAGE ID | spotted DNA/cDNA | 94% | 94% |
| GPL3524 | Stanford IMAGE ID | spotted DNA/cDNA | 94% | 94% |
| GPL3528 | Stanford IMAGE ID | spotted DNA/cDNA | 92% | 92% |
| GPL3895 | Stanford IMAGE ID | spotted DNA/cDNA | 97% | 97% |
| GPL3898 | Stanford IMAGE ID | spotted DNA/cDNA | 92% | 92% |
| GPL4482 | Stanford IMAGE ID | spotted DNA/cDNA | 81% | 81% |
| GPL4483 | Stanford IMAGE ID | spotted DNA/cDNA | 92% | 92% |
| GPL4505 | Stanford IMAGE ID | spotted DNA/cDNA | 77% | 77% |
| GPL4639 | Stanford IMAGE ID | spotted DNA/cDNA | 94% | 94% |
| GPL4640 | Stanford IMAGE ID | spotted DNA/cDNA | 94% | 94% |
| GPL5620 | Stanford IMAGE ID | spotted DNA/cDNA | 94% | 94% |
| GPL6317 | Stanford IMAGE ID | spotted DNA/cDNA | 92% | 92% |
| GPL6318 | Stanford IMAGE ID | spotted DNA/cDNA | 94% | 94% |
| GPL6319 | Stanford IMAGE ID | spotted DNA/cDNA | 97% | 97% |
| GPL6320 | Stanford IMAGE ID | spotted DNA/cDNA | 97% | 97% |
| GPL6321 | Stanford IMAGE ID | spotted DNA/cDNA | 97% | 97% |
| GPL6322 | Stanford IMAGE ID | spotted DNA/cDNA | 94% | 94% |
| GPL6323 | Stanford IMAGE ID | spotted DNA/cDNA | 94% | 94% |
| GPL6468 | Stanford IMAGE ID | spotted DNA/cDNA | 94% | 94% |
| GPL7321 | Stanford IMAGE ID | spotted DNA/cDNA | 86% | 86% |
| GPL7322 | Stanford IMAGE ID | spotted DNA/cDNA | 84% | 84% |
| GPL7323 | Stanford IMAGE ID | spotted DNA/cDNA | 86% | 86% |
| GPL7324 | Stanford IMAGE ID | spotted DNA/cDNA | 86% | 86% |
| GPL7325 | Stanford IMAGE ID | spotted DNA/cDNA | 86% | 86% |
| GPL7778 | Stanford IMAGE ID | spotted DNA/cDNA | 86% | 86% |
| GPL7779 | Stanford IMAGE ID | spotted DNA/cDNA | 86% | 86% |
| GPL7780 | Stanford IMAGE ID | spotted DNA/cDNA | 86% | 86% |
| GPL7781 | Stanford IMAGE ID | spotted DNA/cDNA | 84% | 84% |
| GPL7782 | Stanford IMAGE ID | spotted DNA/cDNA | 86% | 86% |
| GPL7783 | Stanford IMAGE ID | spotted DNA/cDNA | 83% | 83% |
| GPL7784 | Stanford IMAGE ID | spotted DNA/cDNA | 86% | 86% |
| GPL8641 | Stanford IMAGE ID | spotted DNA/cDNA | 82% | 82% |

|           |                         |      |     |      |
|-----------|-------------------------|------|-----|------|
| GPL 10093 | spotted DNA/cDNA        | NA   | NA  | NA   |
| GPL 1424  | spotted DNA/cDNA        | 100% |     | 100% |
| GPL 1506  | spotted DNA/cDNA        | 87%  |     | 96%  |
| GPL 3632  | spotted DNA/cDNA        | 99%  | 9%  | 99%  |
| GPL 3887  | spotted DNA/cDNA        | 100% |     | 100% |
| GPL 3888  | spotted DNA/cDNA        | 99%  |     | 99%  |
| GPL 3889  | spotted DNA/cDNA        | 100% |     | 100% |
| GPL 3892  | spotted DNA/cDNA        | 86%  | 10% | 96%  |
| GPL 3893  | spotted DNA/cDNA        | 99%  |     | 99%  |
| GPL 3894  | spotted DNA/cDNA        | 89%  | 10% | 99%  |
| GPL 4003  | spotted DNA/cDNA        | 100% |     | 100% |
| GPL 4242  | spotted DNA/cDNA        | 100% |     | 100% |
| GPL 4453  | spotted DNA/cDNA        | NA   | NA  | NA   |
| GPL 4998  | spotted DNA/cDNA        | 100% |     | 100% |
| GPL 4999  | spotted DNA/cDNA        | 100% |     | 100% |
| GPL 5749  | spotted DNA/cDNA        | 99%  |     | 99%  |
| GPL 5750  | spotted DNA/cDNA        | 99%  |     | 99%  |
| GPL 6359  | spotted DNA/cDNA        | 99%  |     | 99%  |
| GPL 6365  | spotted DNA/cDNA        | 100% |     | 100% |
| GPL 8999  | spotted DNA/cDNA        | 100% |     | 100% |
| GPL 9189  | spotted DNA/cDNA        | 99%  |     | 99%  |
| GPL 5046  | spotted oligonucleotide | 100% |     | 100% |
| GPL 2819  | spotted oligonucleotide | 96%  |     | 96%  |
| GPL 2826  | spotted oligonucleotide | 96%  |     | 96%  |
| GPL 2827  | spotted oligonucleotide | 97%  |     | 97%  |
| GPL 2834  | spotted oligonucleotide | 96%  |     | 96%  |
| GPL 3055  | spotted oligonucleotide | 96%  |     | 96%  |
| GPL 5149  | spotted oligonucleotide | 100% |     | 100% |
| GPL 5326  | spotted oligonucleotide | 100% |     | 100% |
| GPL 5711  | spotted oligonucleotide | 100% |     | 100% |
| GPL 8276  | spotted oligonucleotide | 100% |     | 100% |
| GPL 8368  | spotted oligonucleotide | 100% |     | 100% |
| GPL 8876  | spotted oligonucleotide | 96%  | 2%  | 98%  |
| GPL 10452 | spotted oligonucleotide | NA   | NA  | NA   |

|          |      |                                |     |    |    |     |
|----------|------|--------------------------------|-----|----|----|-----|
| GPL5144  | HG18 | spotted oligonucleotide        | NA  | NA | NA | NA  |
| GPL5737  | HG18 | spotted oligonucleotide        | NA  | NA | NA | NA  |
| GPL9852  | HG18 | spotted oligonucleotide        | NA  | NA | NA | NA  |
| GPL10001 |      | spotted oligonucleotide        | NA  | NA | NA | NA  |
| GPL9216  |      | spotted oligonucleotide        | NA  | NA | NA | NA  |
| GPL3054  | HG16 | spotted oligonucleotide/BAC/P1 | 94% |    |    | 94% |

**Supplementary Table S5: Normal tissue reference arrays for Affymetrix platforms**

| <b>Affymetrix platform</b> | <b>GSM_ID</b> |
|----------------------------|---------------|
| GenomeWideSNP_6            | GSM397671     |
|                            | GSM397705     |
|                            | GSM397707     |
|                            | GSM397727     |
|                            | GSM397731     |
|                            | GSM397745     |
|                            | GSM397747     |
|                            | GSM397748     |
|                            | GSM397750     |
|                            | GSM397752     |
|                            | GSM397760     |
|                            | GSM397762     |
|                            | GSM397766     |
|                            | GSM397767     |
|                            | GSM397778     |
|                            | GSM397794     |
|                            | GSM397807     |
|                            | GSM397808     |
|                            | GSM397814     |
|                            | GSM397821     |
|                            | GSM397822     |
|                            | GSM397823     |
|                            | GSM397824     |
|                            | GSM397826     |
|                            | GSM397831     |
|                            | GSM397833     |
|                            | GSM397834     |
|                            | GSM397835     |
|                            | GSM397838     |
|                            | GSM457680     |
|                            | GSM457682     |
|                            | GSM457686     |
|                            | GSM457688     |
|                            | GSM457690     |
|                            | GSM457693     |
|                            | GSM457708     |
|                            | GSM457712     |
|                            | GSM457714     |
|                            | GSM457716     |
|                            | GSM457719     |
|                            | GSM457721     |
|                            | GSM457723     |
|                            | GSM457731     |
|                            | GSM457741     |
|                            | GSM457747     |
|                            | GSM457750     |
|                            | GSM540611     |
|                            | GSM540624     |
|                            | GSM540625     |
|                            | GSM540640     |
| Mapping250K_Nsp            | GSM317821     |

GSM317824

GSM353474

GSM353475

GSM353476

GSM353477

GSM353478

GSM353479

GSM353480

GSM353481

GSM353489

GSM353491

GSM353493

GSM393578

GSM393579

GSM503448

GSM503449

GSM503452

GSM503455

GSM503456

GSM503457

GSM503459

GSM503460

GSM503461

GSM503462

GSM503463

GSM503465

GSM503467

GSM503468

GSM503469

GSM503472

GSM503473

GSM503672

GSM503673

GSM503674

GSM503675

GSM503678

GSM503682

GSM503683

GSM503686

GSM503689

GSM503690

GSM503691

GSM503693

GSM503694

GSM503695

GSM503696

GSM503697

GSM503698

GSM503699

Mapping250K\_Sty

GSM372871

GSM372872

GSM372875

GSM372876

GSM372877

GSM372878

|                    |           |
|--------------------|-----------|
|                    | GSM372880 |
|                    | GSM372881 |
|                    | GSM372882 |
|                    | GSM372883 |
|                    | GSM372884 |
|                    | GSM372885 |
|                    | GSM372886 |
|                    | GSM372887 |
|                    | GSM372889 |
|                    | GSM372892 |
|                    | GSM372893 |
|                    | GSM372894 |
|                    | GSM372896 |
|                    | GSM372897 |
|                    | GSM372898 |
|                    | GSM374507 |
|                    | GSM374517 |
|                    | GSM374518 |
|                    | GSM374520 |
|                    | GSM374524 |
|                    | GSM374525 |
|                    | GSM374526 |
|                    | GSM374527 |
|                    | GSM503534 |
|                    | GSM503541 |
|                    | GSM503542 |
|                    | GSM503543 |
|                    | GSM503546 |
|                    | GSM503550 |
|                    | GSM503551 |
|                    | GSM503553 |
|                    | GSM503554 |
|                    | GSM503555 |
|                    | GSM503556 |
|                    | GSM503557 |
|                    | GSM503558 |
|                    | GSM503559 |
|                    | GSM503560 |
|                    | GSM503563 |
|                    | GSM529110 |
|                    | GSM529112 |
|                    | GSM529113 |
|                    | GSM529115 |
|                    | GSM529129 |
| Mapping50K_Hind240 | GSM173736 |
|                    | GSM173737 |
|                    | GSM173738 |
|                    | GSM173739 |
|                    | GSM173742 |
|                    | GSM173743 |
|                    | GSM173744 |
|                    | GSM173745 |
|                    | GSM173755 |
|                    | GSM173756 |
|                    | GSM173757 |

|                   |           |
|-------------------|-----------|
|                   | GSM173760 |
|                   | GSM173761 |
|                   | GSM173762 |
|                   | GSM173767 |
|                   | GSM173768 |
|                   | GSM173774 |
|                   | GSM173775 |
|                   | GSM173777 |
|                   | GSM173778 |
|                   | GSM173779 |
|                   | GSM173780 |
|                   | GSM173782 |
|                   | GSM173785 |
|                   | GSM173787 |
|                   | GSM173793 |
|                   | GSM173794 |
|                   | GSM173795 |
|                   | GSM173799 |
|                   | GSM173800 |
|                   | GSM173804 |
|                   | GSM173805 |
|                   | GSM174872 |
|                   | GSM190405 |
|                   | GSM190406 |
|                   | GSM190407 |
|                   | GSM190408 |
|                   | GSM248616 |
|                   | GSM248617 |
|                   | GSM248619 |
|                   | GSM248620 |
|                   | GSM248621 |
|                   | GSM248623 |
|                   | GSM248624 |
|                   | GSM248629 |
|                   | GSM248640 |
| Mapping50K_Xba240 | GSM288038 |
|                   | GSM288048 |
|                   | GSM288050 |
|                   | GSM288052 |
|                   | GSM288054 |
|                   | GSM288056 |
|                   | GSM288058 |
|                   | GSM288060 |
|                   | GSM288062 |
|                   | GSM288068 |
|                   | GSM288070 |
|                   | GSM288072 |
|                   | GSM288076 |
|                   | GSM288078 |
|                   | GSM288082 |
|                   | GSM288084 |
|                   | GSM288086 |
|                   | GSM288092 |
|                   | GSM288094 |

|                   |           |
|-------------------|-----------|
|                   | GSM288096 |
|                   | GSM288100 |
|                   | GSM288104 |
|                   | GSM288106 |
|                   | GSM288108 |
|                   | GSM288118 |
|                   | GSM288122 |
|                   | GSM288124 |
|                   | GSM288126 |
|                   | GSM288128 |
|                   | GSM288136 |
|                   | GSM288142 |
|                   | GSM288146 |
|                   | GSM288152 |
|                   | GSM288158 |
|                   | GSM288160 |
|                   | GSM288164 |
|                   | GSM288166 |
|                   | GSM288178 |
|                   | GSM288184 |
|                   | GSM288186 |
|                   | GSM288192 |
|                   | GSM288194 |
|                   | GSM288198 |
|                   | GSM288204 |
|                   | GSM288206 |
|                   | GSM288210 |
|                   | GSM288214 |
|                   | GSM288216 |
|                   | GSM288218 |
|                   | GSM288222 |
| Mapping10K_Xba131 | GSM85243  |
|                   | GSM85244  |
|                   | GSM85245  |
|                   | GSM85249  |
|                   | GSM85251  |
|                   | GSM85255  |
|                   | GSM85257  |
|                   | GSM85264  |
|                   | GSM85265  |
|                   | GSM85266  |
|                   | GSM85267  |
|                   | GSM488268 |
|                   | GSM488269 |
|                   | GSM488270 |
|                   | GSM488273 |
|                   | GSM488274 |
|                   | GSM488275 |
|                   | GSM488276 |
|                   | GSM488277 |
|                   | GSM488280 |
|                   | GSM488281 |
|                   | GSM488282 |
|                   | GSM488283 |
|                   | GSM488284 |
|                   | GSM488286 |

|                   |           |
|-------------------|-----------|
|                   | GSM488289 |
|                   | GSM488290 |
|                   | GSM488291 |
|                   | GSM488292 |
|                   | GSM488296 |
|                   | GSM488297 |
|                   | GSM488299 |
|                   | GSM488301 |
|                   | GSM488303 |
| Mapping10K_Xba142 | GSM163110 |
|                   | GSM163128 |
|                   | GSM163152 |
|                   | GSM163163 |
|                   | GSM163182 |
|                   | GSM163207 |
|                   | GSM163234 |
|                   | GSM163240 |
|                   | GSM163246 |
|                   | GSM163247 |
|                   | GSM163259 |
|                   | GSM163268 |
|                   | GSM163283 |
|                   | GSM163305 |
|                   | GSM163323 |
|                   | GSM163325 |
|                   | GSM163343 |
|                   | GSM163354 |
|                   | GSM163370 |
|                   | GSM163373 |
|                   | GSM163388 |
|                   | GSM163407 |
|                   | GSM163417 |
|                   | GSM163424 |
|                   | GSM163426 |
|                   | GSM163442 |
|                   | GSM163462 |
|                   | GSM163466 |
|                   | GSM163478 |
|                   | GSM163494 |
|                   | GSM163515 |
|                   | GSM163516 |
|                   | GSM163537 |
|                   | GSM163538 |
|                   | GSM163547 |
|                   | GSM163566 |
|                   | GSM163579 |
|                   | GSM163600 |
|                   | GSM163613 |
|                   | GSM163723 |
|                   | GSM163744 |
|                   | GSM163767 |
|                   | GSM163823 |
|                   | GSM163837 |
|                   | GSM163848 |
|                   | GSM216336 |
|                   | GSM216343 |
|                   | GSM243156 |

GSM438329  
GSM438345
